# Supplementary material for: Geometric Modeling of Hippocampal Tau Deposition: A Surface-Based Framework for Covariate Analysis and Off-Target Contamination Detection
Source: arXiv:2511.01732 source file (2026-09-01)
Supplement: Supplementary file 1 [file Supplementary.tex]

\documentclass{article}
\usepackage{graphicx}
\usepackage{caption}
\usepackage{subcaption}
\usepackage{amsmath}
\usepackage{geometry}
\usepackage{hyperref}
\usepackage{float}
\usepackage{booktabs}
\usepackage{natbib}
\usepackage[section]{placeins}

\geometry{margin=1in}
\setlength{\parskip}{1em}
\setlength{\parindent}{0em}

\title{Supplementary Figures}
\begin{document}

\maketitle

\begin{figure}[h!]
    \centering
    \includegraphics[width=14cm]{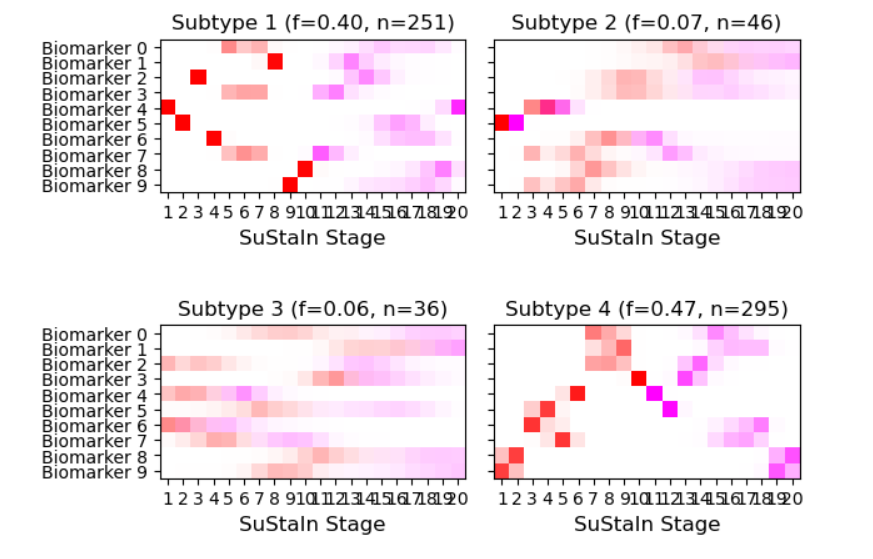}
    \caption{SuStaIn output matched with PVD plot}
    \label{fig: sustain_pvd}
\end{figure}

\section{Directional consistency validation}
\subsection{Principal Surface Selection} \label{sec: Principal Surface Selection}

To ensure that the principal surface (PS) provides an accurate and stable representation of tau deposition without overfitting, we evaluate its smoothness and geometric consistency using Gaussian curvature (\( K_i \)). High curvature regions indicate potential overfitting, where the surface captures noise rather than meaningful structural variations. To mitigate this, we apply curvature-based filtering to prevent self-intersections and excessive flexibility in the PS fitting process, ensuring a stable yet representative surface.

Gaussian curvature is computed at each surface point \( \mathbf{q}_i = (x_i, y_i, z_i) = f(t_{1i}, t_{2i}) \) using the first and second fundamental forms:
\[
\mathbf{K}_i = \frac{\mathbf{L}_i \mathbf{N}_i - \mathbf{M}_i^2}{\mathbf{E}_i \mathbf{G}_i - \mathbf{F}_i^2}.
\]
where \( \mathbf{E}_i, \mathbf{F}_i, \mathbf{G}_i \) define local metric properties:
\[
  \mathbf{E}_i = \left\| \frac{\partial f}{\partial t_{1i}} \right\|^2, \quad 
  \mathbf{F}_i = \frac{\partial f}{\partial t_{1i}} \cdot \frac{\partial f}{\partial t_{2i}}, \quad 
  \mathbf{G}_i = \left\| \frac{\partial f}{\partial t_{2i}} \right\|^2,
\]
and \( \mathbf{L}_i, \mathbf{M}_i, \mathbf{N}_i \) capture curvature variations:
\[
  \mathbf{L}_i = \mathcal{N}_i \cdot \frac{\partial^2 f}{\partial t_{1i}^2}, \quad 
  \mathbf{M}_i = \mathcal{N}_i \cdot \frac{\partial^2 f}{\partial t_{1i} \partial t_{2i}}, \quad 
  \mathbf{N}_i = \mathcal{N}_i \cdot \frac{\partial^2 f}{\partial t_{2i}^2}.
\]

The unit normal vector \( \mathcal{N}_i \) at each point is computed as the cross product of the tangent vectors:
\[
\mathcal{N}_i = \frac{\partial f}{\partial t_{1i}} \times \frac{\partial f}{\partial t_{2i}}.
\]
To ensure numerical stability, derivatives are approximated using finite differences:
\[
\frac{\partial f}{\partial t_{1i}} \approx \frac{f(t_{1i}+h, t_{2i}) - f(t_{1i}-h, t_{2i})}{2h},
\]
\[
\frac{\partial^2 f}{\partial t_{1i} \partial t_{2i}} \approx \frac{f(t_{1i}+h, t_{2i}+h) - f(t_{1i}+h, t_{2i}-h) - f(t_{1i}-h, t_{2i}+h) + f(t_{1i}-h, t_{2i}-h)}{4h^2}.
\]

By analyzing the distribution of curvature values, we discard PS candidates with excessive local curvature that could lead to artifacts. The final selected surface balances smoothness and structural representation, ensuring a robust framework for subsequent tau deposition analysis.

\subsection{Projection Vectors Difference}

This representation assumes that the intrinsic normal vectors of the PS are well aligned with the projection directions from hippocampal boundaries. That is, when projecting a voxel from the boundary onto the PS (for distance computation or SUVR interpolation), the resulting vector should approximate the PS normal at the target point. While this holds in most regions, local misalignment may occur in areas of high curvature due to numerical approximation of normals (via finite differences) or the shortest-path projection strategy. The misalignment of two projection vectors can be found in Supplementary Figure S2.

\begin{figure}[htbp]
    \centering
    \begin{tabular}{cc}
        \includegraphics[width=0.45\textwidth]{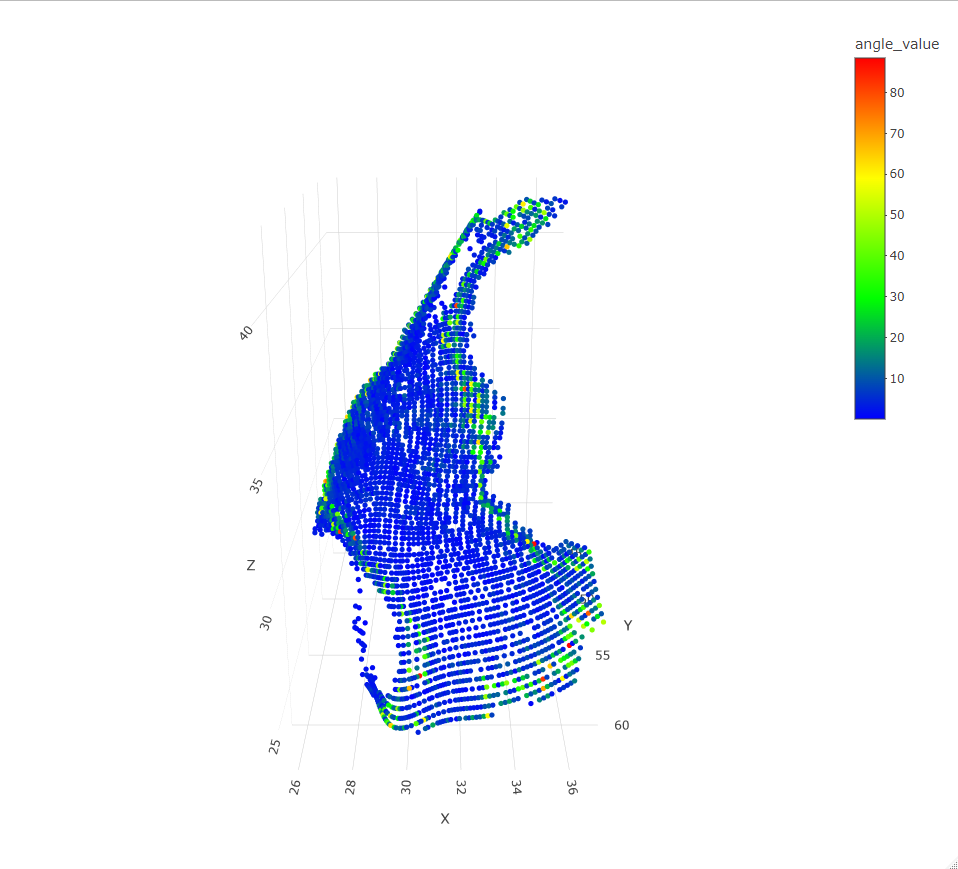} &
        \includegraphics[width=0.45\textwidth]{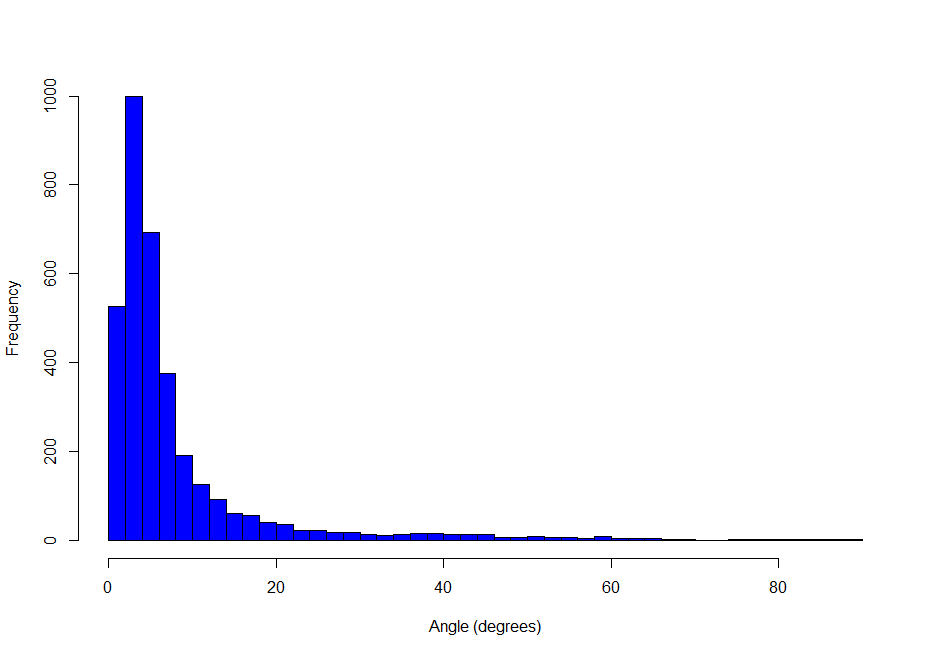} \\
        (a) 3D Angle Distribution Map & (b) Angle Distribution Histogram \\

    \end{tabular}
    \caption{
Directional consistency validation 
(a) Spatial map of angular differences between projection and normal vectors, showing localized misalignment. 
(b) Histogram of angle deviations confirms strong directional consistency across surface points. 
}
    \label{fig:validation_reconstruction}
\end{figure}

\begin{figure}[h]
    \centering
    \begin{tabular}{cc}
        \includegraphics[width=0.45\textwidth]{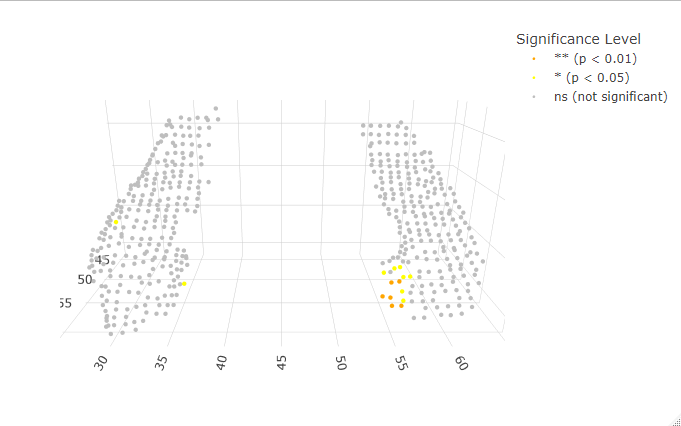} &
        \includegraphics[width=0.45\textwidth]{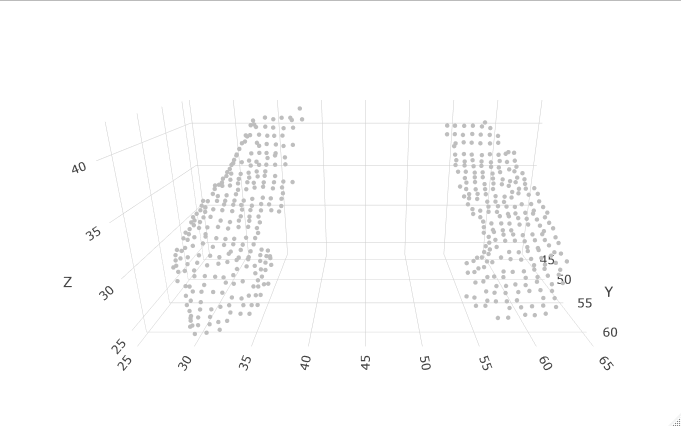} 
        \\
        (a) Age effect significance for subtype 1 & (b) Age effect significance for subtype 2
        \\
        \includegraphics[width=0.45\textwidth]{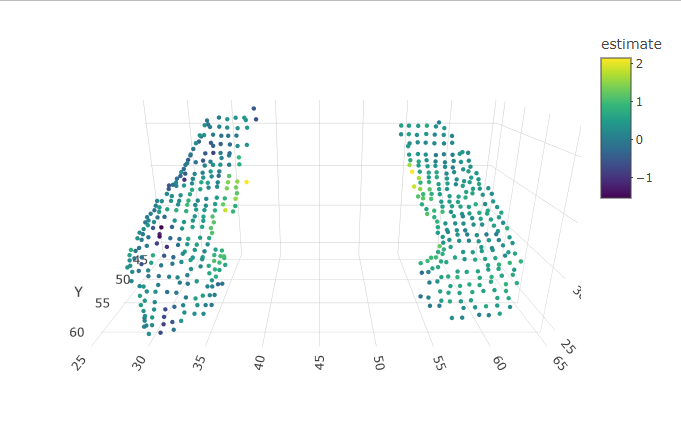} &
        \includegraphics[width=0.45\textwidth]{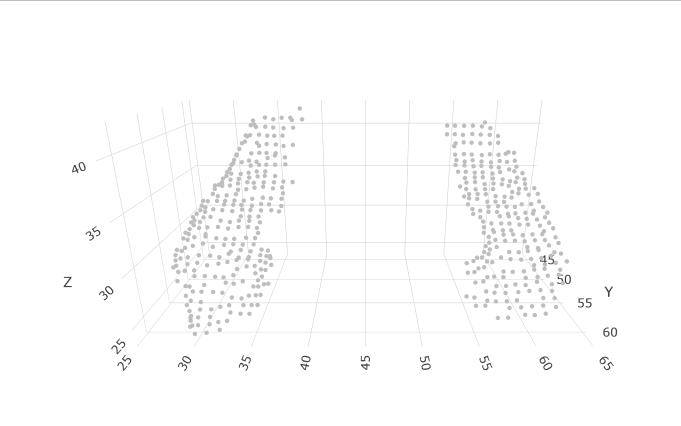} 
        \\
        (c) Sex effect significance for subtype 1 & (d) Sex effect significance for subtype 2
    \end{tabular}
    \caption{Spatial distribution of age and sex effects. }
    \label{fig:spatial_coverage_age_sex}
\end{figure}

\begin{figure}[h]
    \centering
    \begin{tabular}{cc}
        \includegraphics[width=0.45\textwidth]{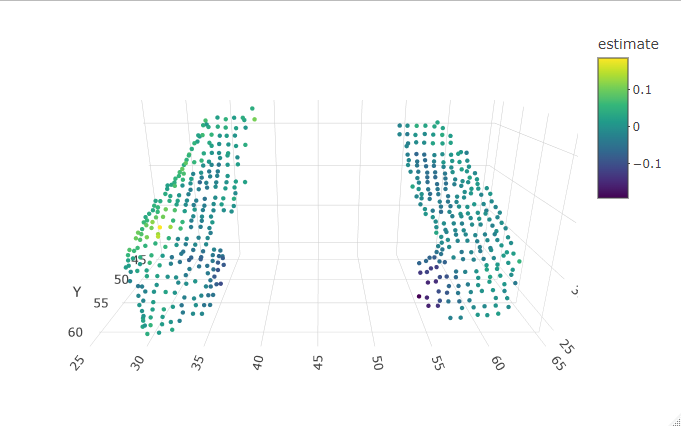}&
        \includegraphics[width=0.45\textwidth]{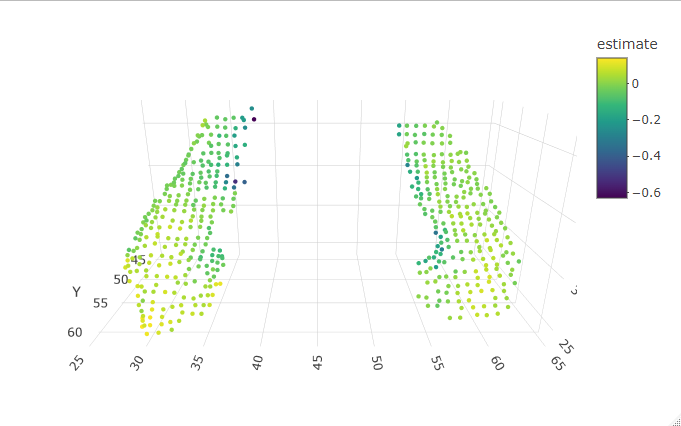} \\
        (a)Age estimate effect for subtype 1  & (b) Age estimate effect for subtype 2 \\
        \includegraphics[width=0.45\textwidth]{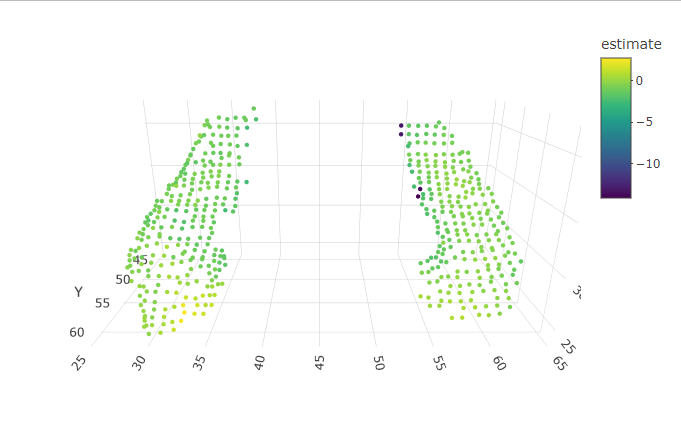}&
        \includegraphics[width=0.45\textwidth]{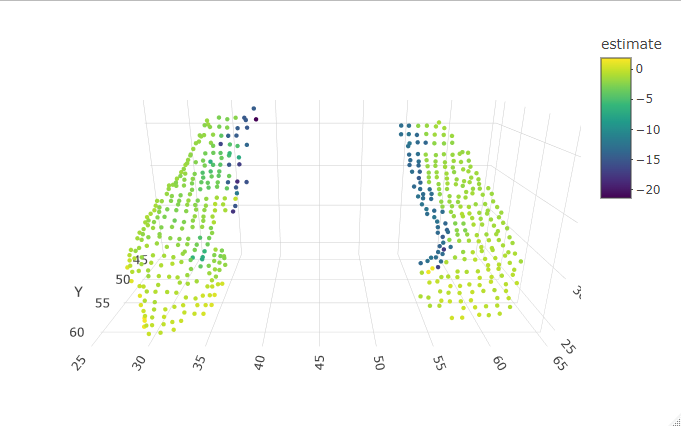} \\
        (c) Diagnosis effect estimate for subtype 1  & (d) Diagnosis effect estimate for subtype 2 \\
        \includegraphics[width=0.45\textwidth]{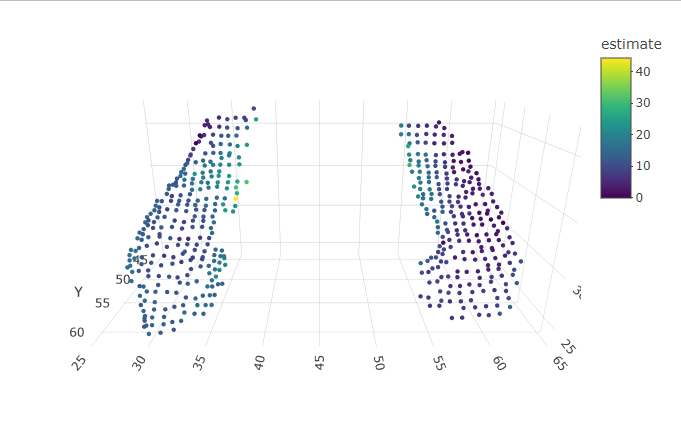} &
        \includegraphics[width=0.45\textwidth]{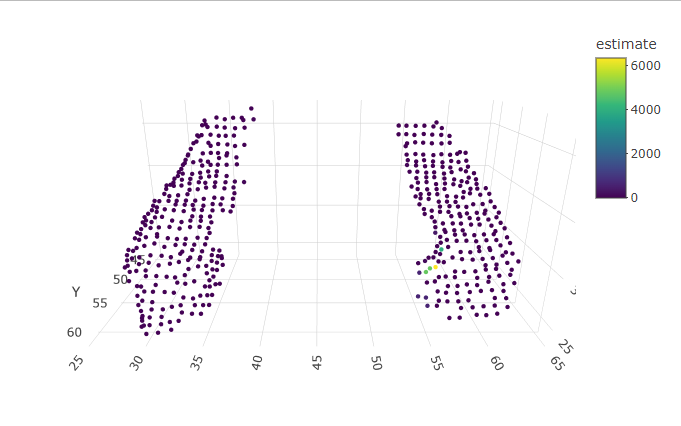} 
        \\
        (e) Linear Stage effect estimate for subtype 1 & (f)  Linear Stage effect for subtype 2
    \end{tabular}
    \caption{Spatial distribution of covariate-associated effects on hippocampal tau coverage across SuStaIn subtypes.
Each panel displays estimated voxel-wise effects (standardized beta coefficients) of age, diagnosis, and SuStaIn stage on hippocampal tau coverage, modeled separately within subtype 1 (left column) and subtype 2 (right column). Notably, age and stage effects show consistent spatial gradients within each subtype, while diagnosis effects differ substantially between subtypes. Subtype 2 exhibits stronger and more localized diagnosis-related effects compared to subtype 1, where diagnosis appears to have limited influence on hippocampal tau distribution. These findings highlight subtype-specific spatial patterns and covariate sensitivities in tau deposition.}
    \label{fig:spatial_coverage_estimate}
\end{figure}

\begin{figure}[h]
    \centering
    \begin{tabular}{cc}
        \includegraphics[width=0.45\textwidth]{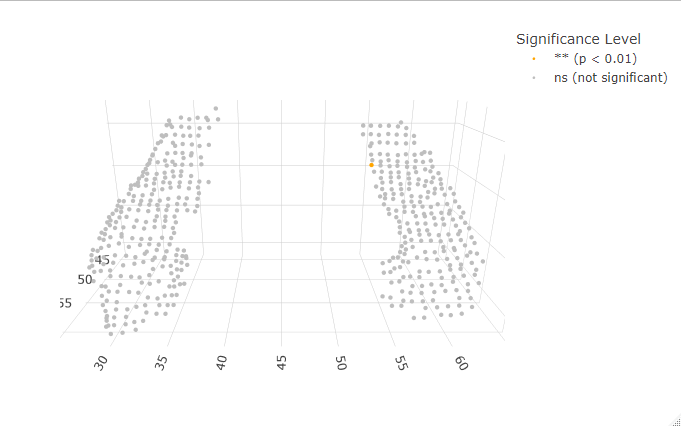}&
        \includegraphics[width=0.45\textwidth]{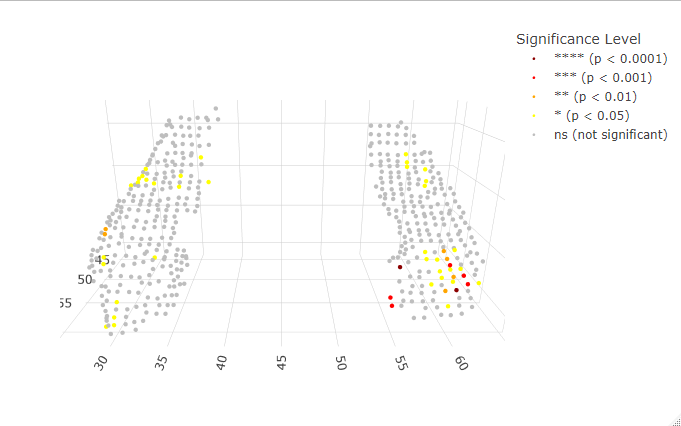} \\ 
        (a)Sex effect significance for subtype 1  & (b)Sex effect significance for subtype 2\\
        \includegraphics[width=0.45\textwidth]{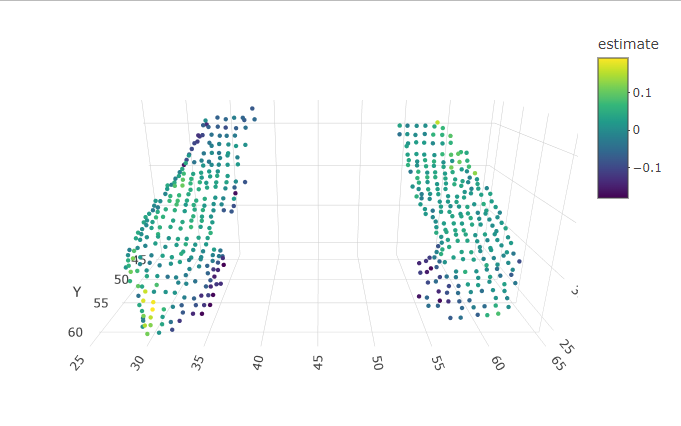}&
        \includegraphics[width=0.45\textwidth]{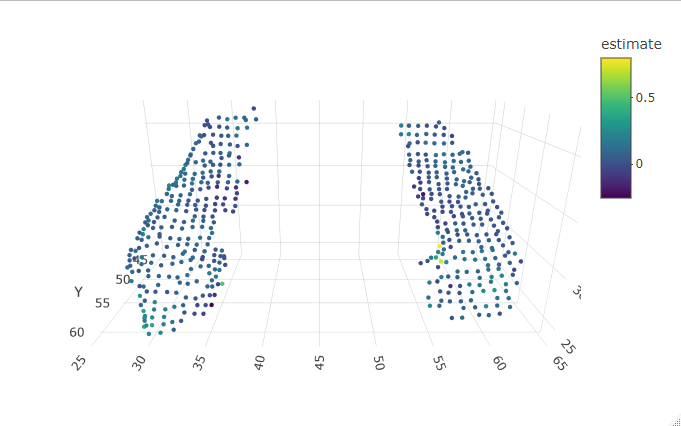} \\
        (c)Sex effect estimate for subtype 1 & (d)Sex effect estimate for subtype 2\\
    \end{tabular}
    \caption{
    Supplementary Figure. Sex-related effects on hippocampal tau SUVR. 
    (a–b) Significance maps for the effect of sex in subtypes 1 and 2. 
    (c–d) Corresponding regression coefficient estimates for each subtype.
    }
    \label{fig:sex_SUVR}
\end{figure}

\begin{figure}[h]
    \centering
    \begin{tabular}{cc}
        \includegraphics[width=0.45\textwidth]{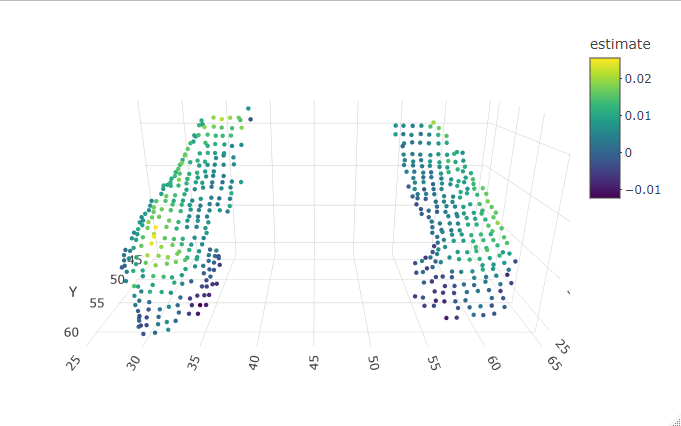}&
        \includegraphics[width=0.45\textwidth]{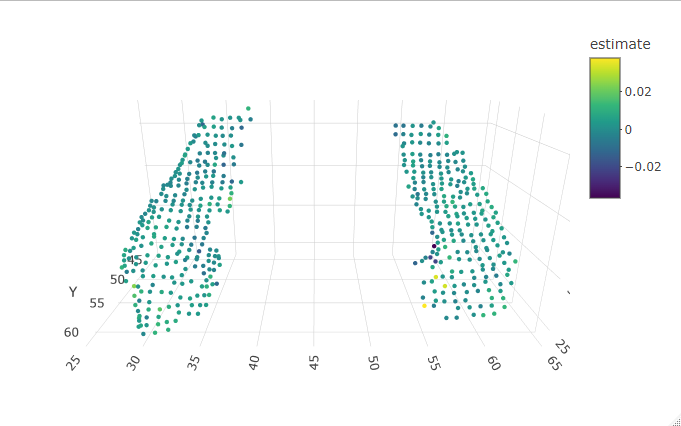} \\ 
        (a) Age estimate for subtype 1  & (b) Age estimate for subtype 2\\
        \includegraphics[width=0.45\textwidth]{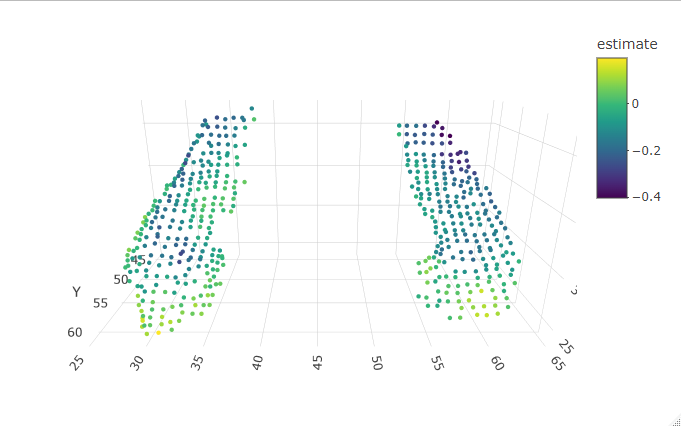}&
        \includegraphics[width=0.45\textwidth]{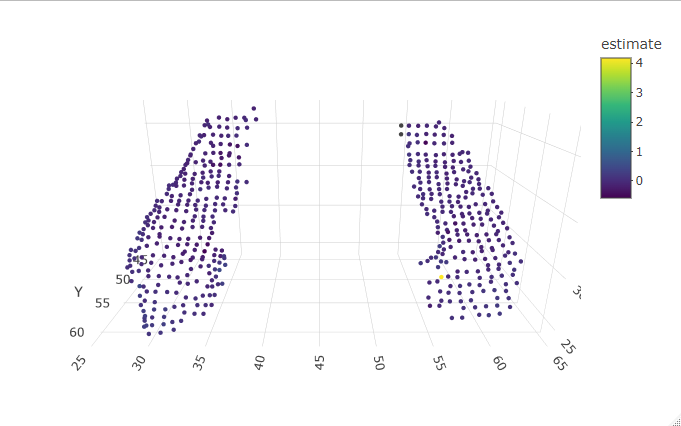} \\
        (c) Diagnosis estimate for subtype 1 & (d) Diagnosis estimate for subtype 2\\
        \includegraphics[width=0.45\textwidth]{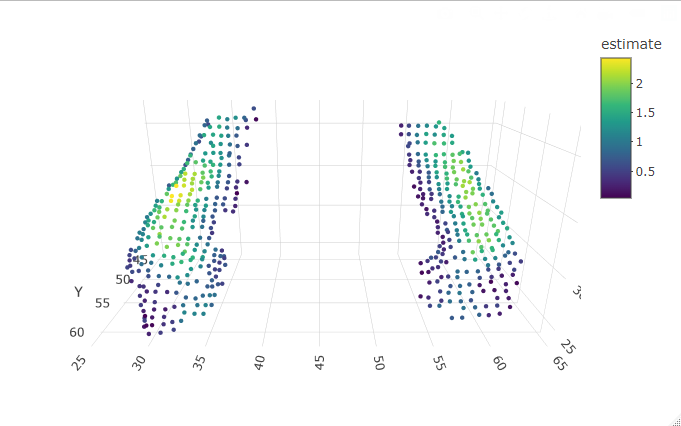}&
        \includegraphics[width=0.45\textwidth]{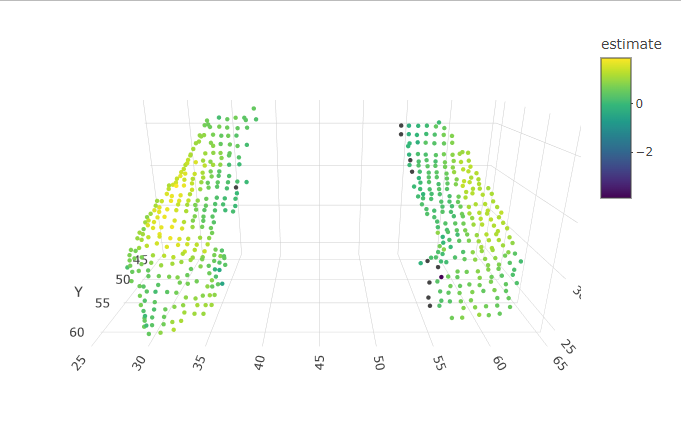} \\
        (e) Linear stage estimate for subtype 1 & (f) Linear stage estimate for subtype 2
    \end{tabular}
    \caption{
    Supplementary Figure. Regression coefficient estimates for covariate effects on hippocampal tau SUVR. 
    (a–b) Age effect estimates. 
    (c–d) Diagnosis effect estimates. 
    (e–f) Linear stage effect estimates, shown separately for subtypes 1 and 2.
    }    
    \label{fig:spatial_SUVR_supp}
\end{figure}

\begin{figure}[h]
    \centering
    \begin{tabular}{cc}
        \includegraphics[width=0.45\textwidth]{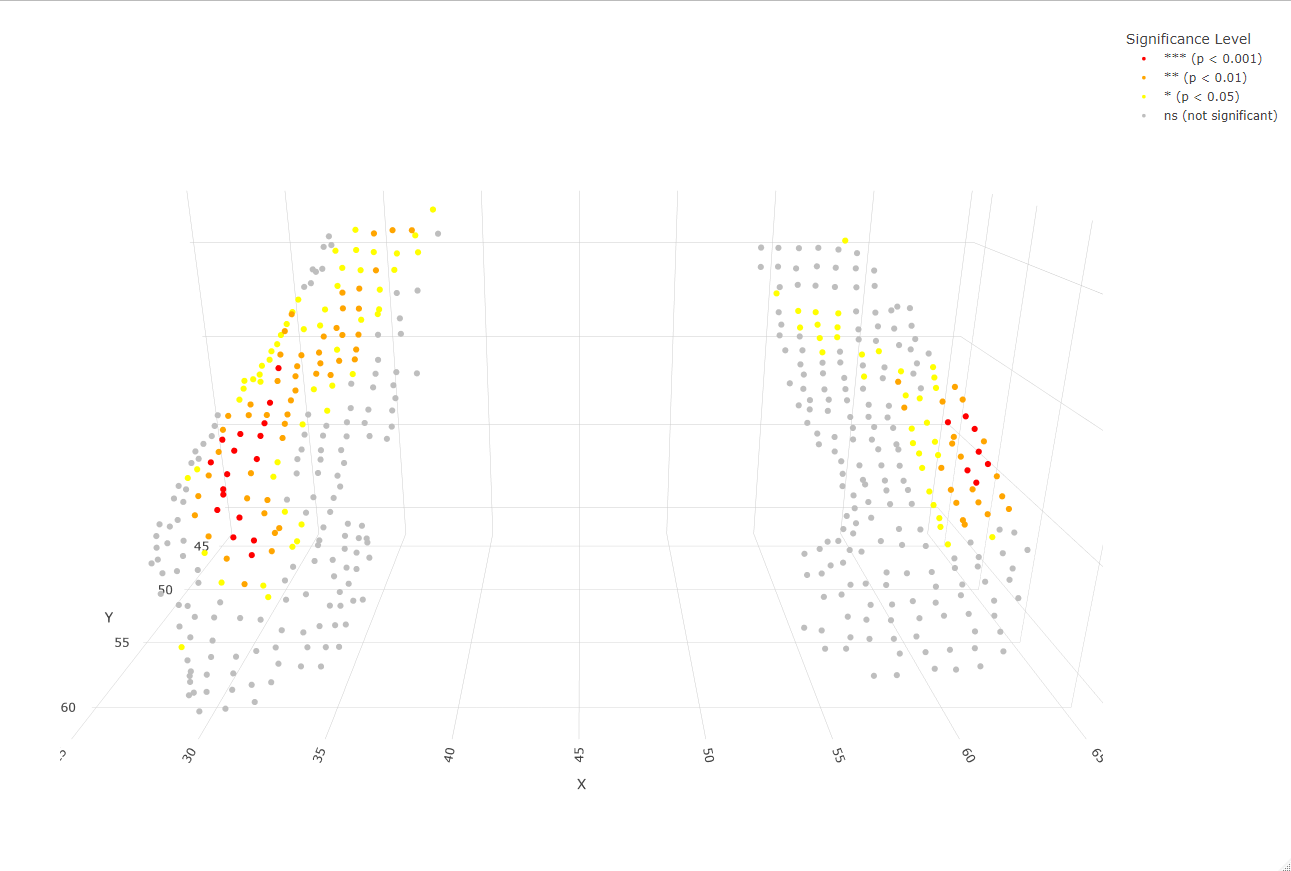}&
        \includegraphics[width=0.45\textwidth]{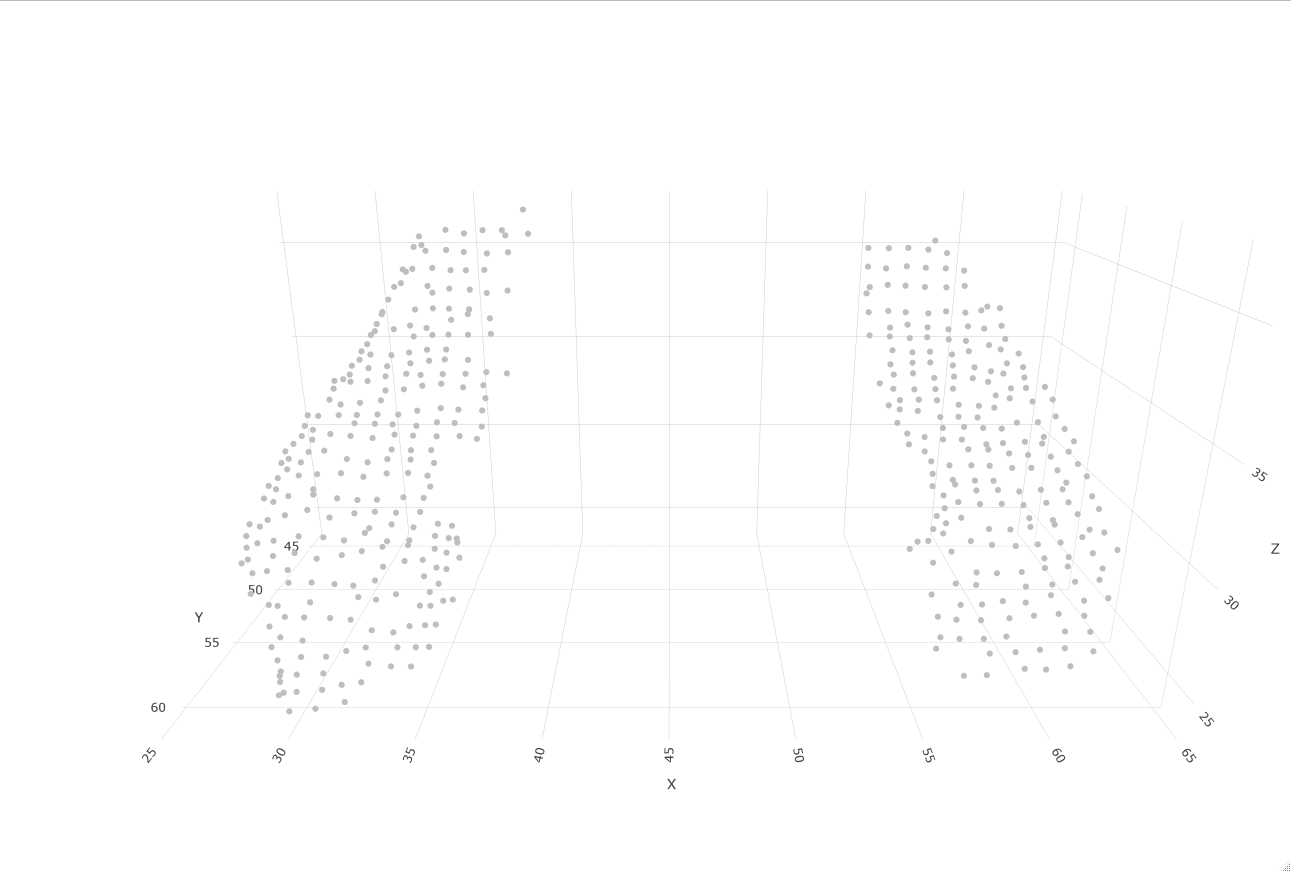} \\ 
        (a)Age significance subtype 1 no IPW & (b)Age significance subtype 2 no IPW\\
        \includegraphics[width=0.45\textwidth]{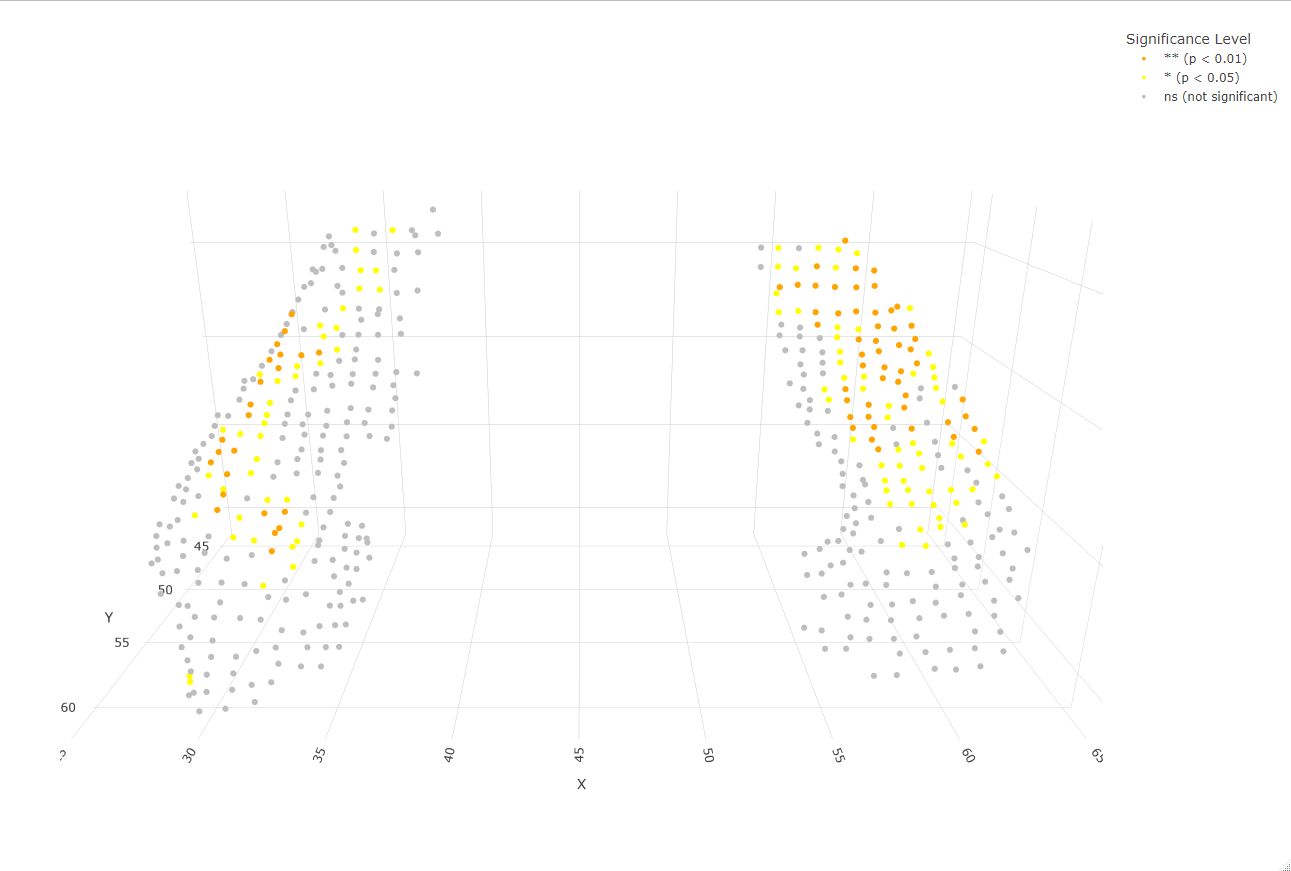}&
        \includegraphics[width=0.45\textwidth]{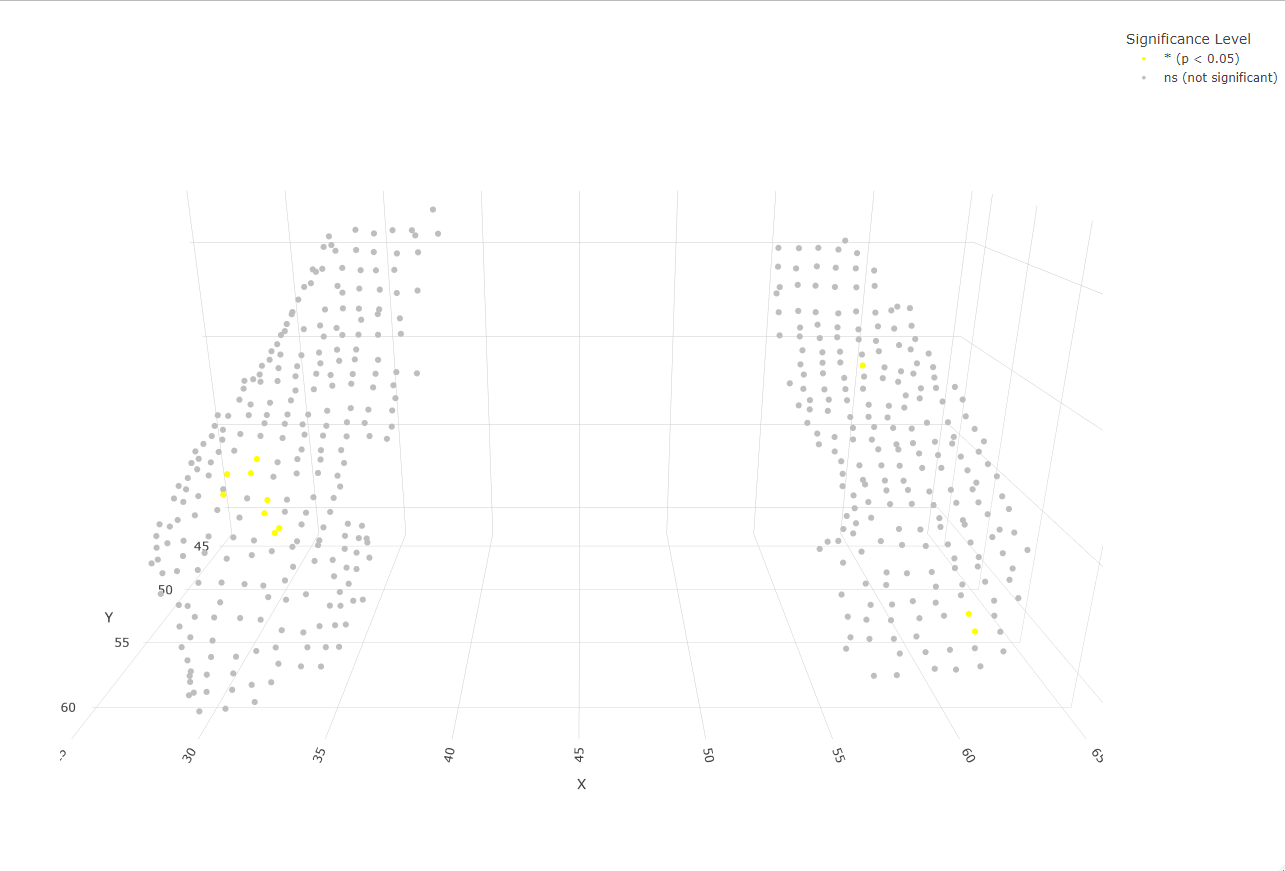} \\
        (c)Diagnosis significance subtype 1 no IPW & (d)Diagnosis significance subtype 2 no IPW\\
    \end{tabular}
    
    \caption{
    Supplementary Figure. Age and Diagnosis-related effects on hippocampal tau SUVR. 
    (a–b) Significance maps for the effect of Age in subtypes 1 and 2 without IPW. 
    (c–d) Significance maps for the effect of Diagnosis in subtypes 1 and 2 without IPW. 
    }
    \label{fig: age_diagnosis_SUVR_no_IPW}
\end{figure}

\begin{figure}[h]
    \centering
    \begin{tabular}{cc}
        \includegraphics[width=0.45\textwidth]{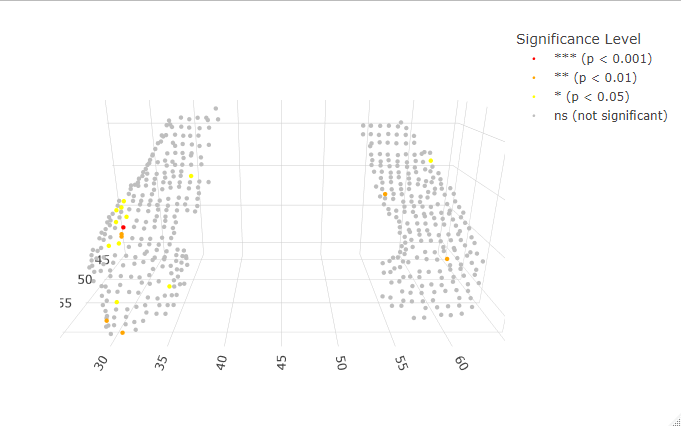} &
        \includegraphics[width=0.45\textwidth]{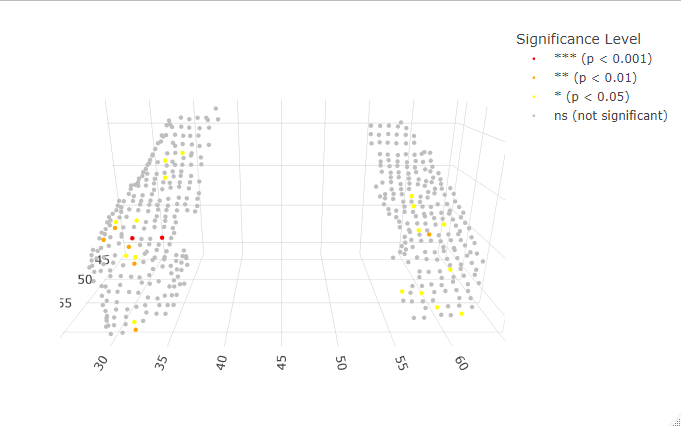} 
        \\
        (a) Age negative distance subtype 1 & (b) Age negative distance for subtype 2
        \\
        \includegraphics[width=0.45\textwidth]{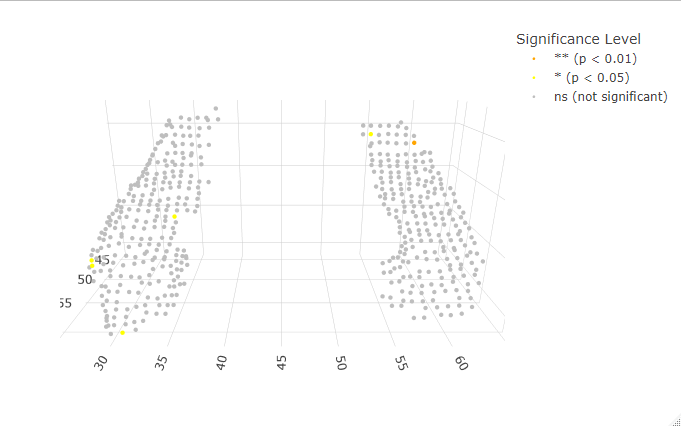} &
        \includegraphics[width=0.45\textwidth]{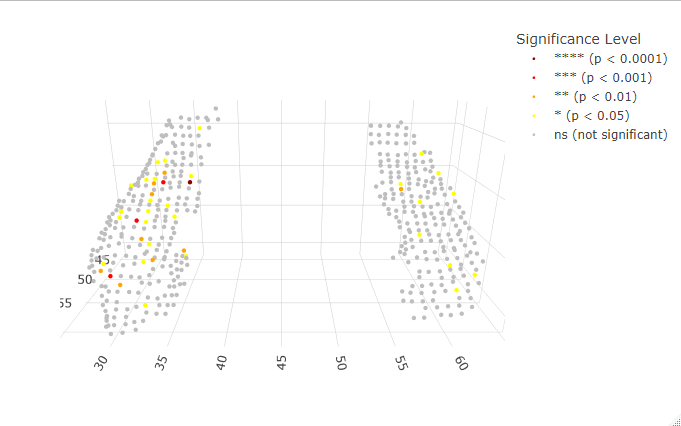} 
        \\
        (c) Diagnosis negative distance subtype 1 & (d) Diagnosis negative distance for subtype 2\\
        \includegraphics[width=0.45\textwidth]{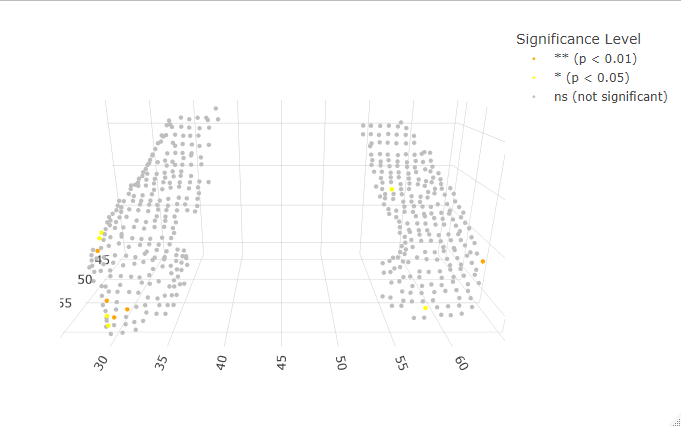} &
        \includegraphics[width=0.45\textwidth]{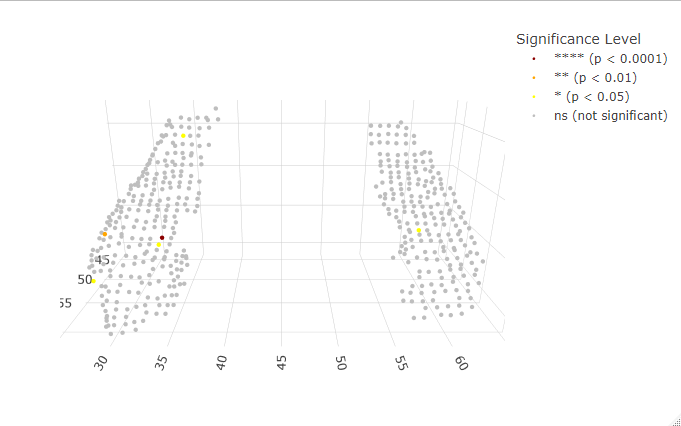} 
        \\
        (e) Sex negative distance subtype 1 & (f) Sex negative distance for subtype 2
    \end{tabular}
    \caption{Thickness of age and diagnosis effects. }
    \label{fig:thickness_age_sex_diagnosis}
\end{figure}

\begin{figure}[h]
    \centering
    \begin{tabular}{cc}
        \includegraphics[width=0.45\textwidth]{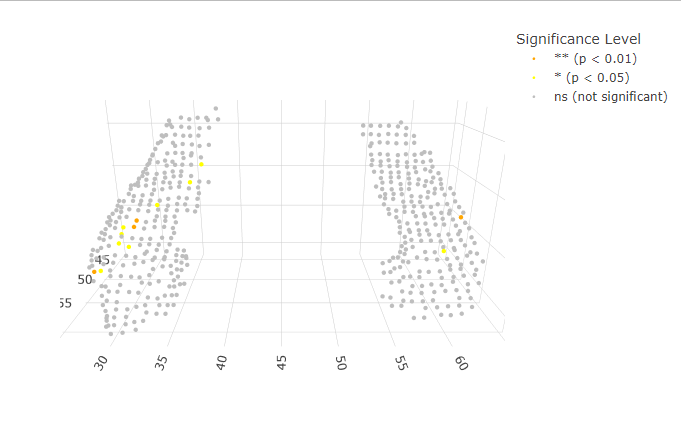} &
        \includegraphics[width=0.45\textwidth]{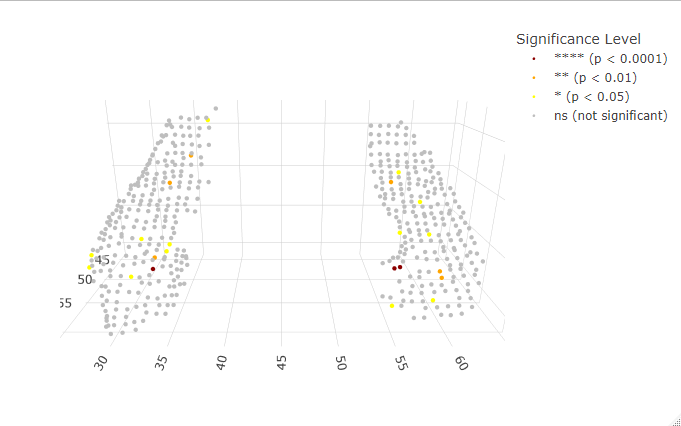} 
        \\
        (a) Age positive distance subtype 1 & (b) Age positive distance for subtype 2
        \\
        \includegraphics[width=0.45\textwidth]{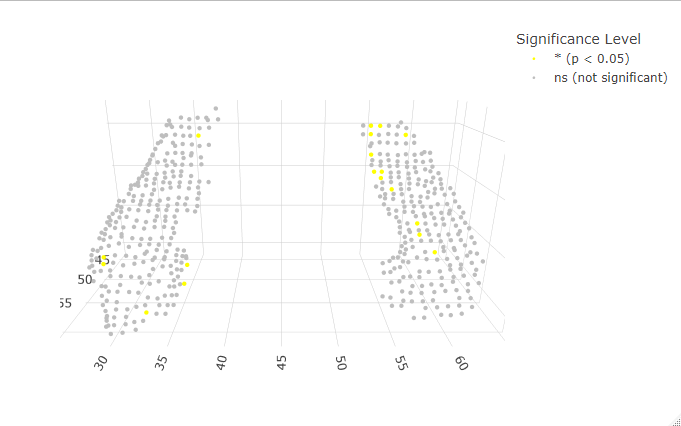} &
        \includegraphics[width=0.45\textwidth]{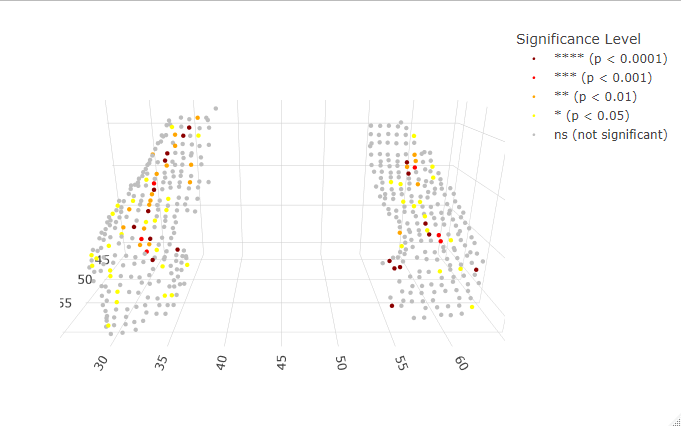} 
        \\
        (c) Diagnosis positive distance subtype 1 & (d) Diagnosis positive distance for subtype 2\\
        \includegraphics[width=0.45\textwidth]{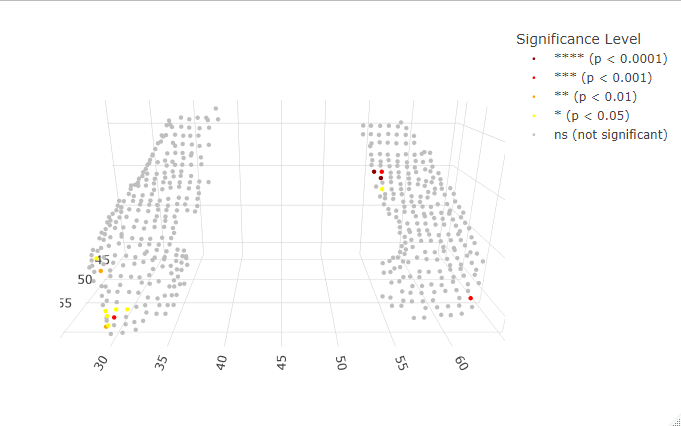} &
        \includegraphics[width=0.45\textwidth]{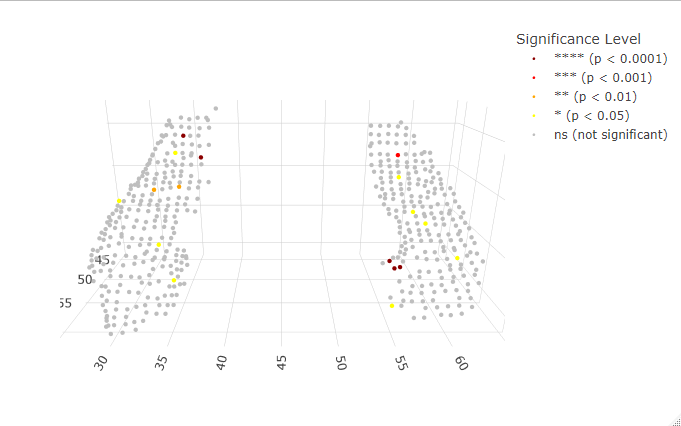} 
        \\
        (e) Diagnosis positive distance subtype 1 & (f) Diagnosis positive distance for subtype 2
    \end{tabular}
    \caption{Thickness of age and diagnosis effects. }
    \label{fig:positive_thickness_age_sex_diagnosis}
\end{figure}

\begin{figure}[h]
    \centering
    \begin{tabular}{cc}
        \includegraphics[width=0.45\textwidth]{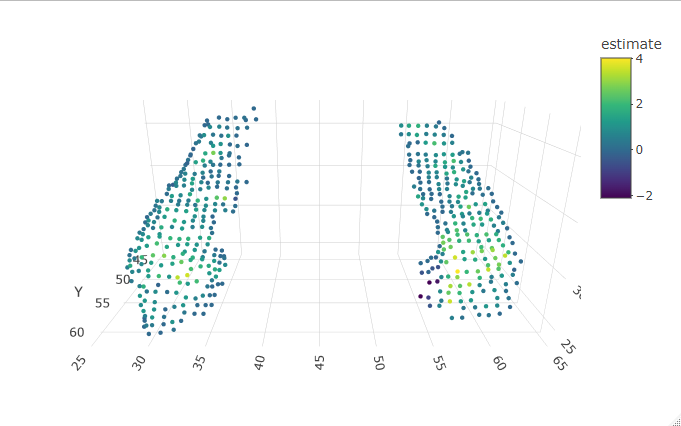}&
        \includegraphics[width=0.45\textwidth]{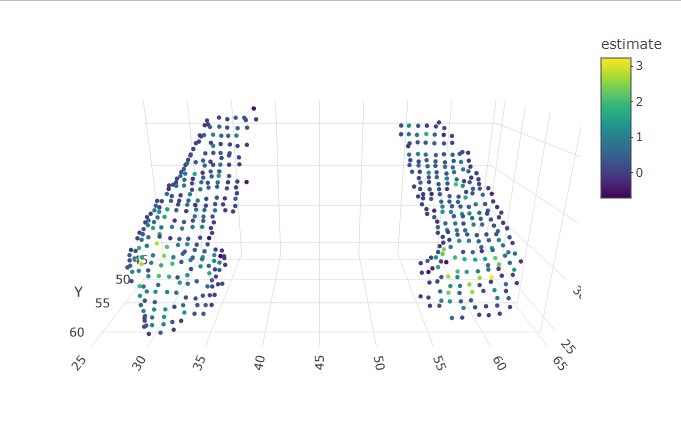} \\ 
        (a) Linear stage estimate subtype 1 negative  & (b) Linear stage estimate subtype 1 positive\\
        \includegraphics[width=0.45\textwidth]{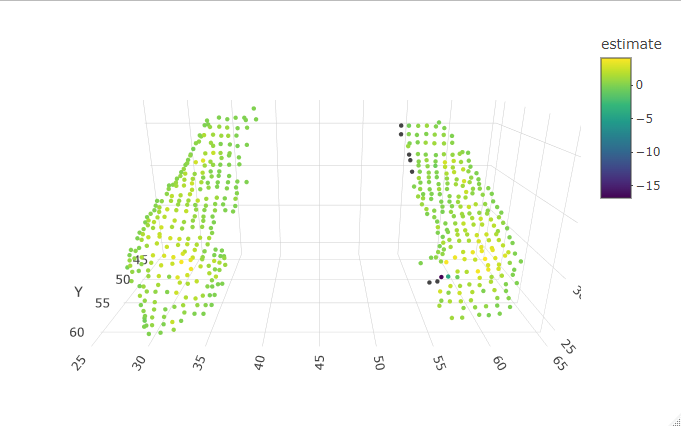}&
        \includegraphics[width=0.45\textwidth]{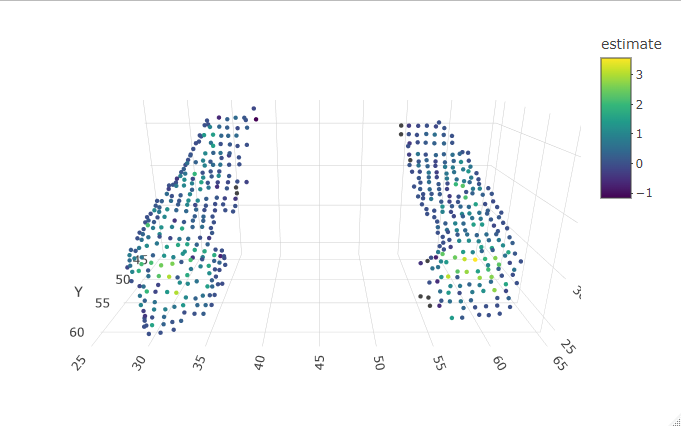} \\
        (c) Linear stage estimate subtype 2 negative & (d) Linear stage estimate subtype 2 positive\\
    \end{tabular}
    \caption{
    Supplementary Figure. SuStaIn stage effects on hippocampal tau deposition thickness, modeled via projection distance features. 
    (a–d) Linear stage coefficient estimates for subtypes 1 and 2, shown separately for negative and positive projection directions. 
    }
\label{fig:thickness_sup}
\end{figure}

\begin{figure}[h]
    \centering
    \begin{tabular}{cc}
        \includegraphics[width=0.45\textwidth]{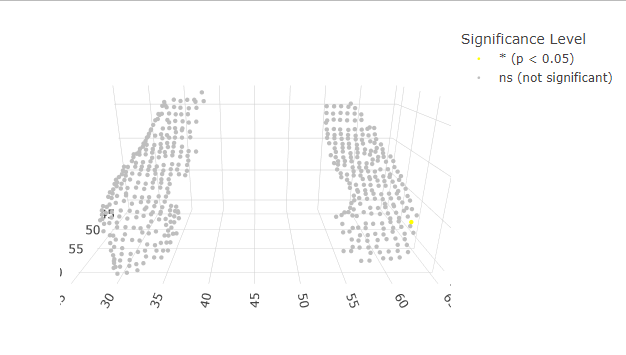}&
        \includegraphics[width=0.45\textwidth]{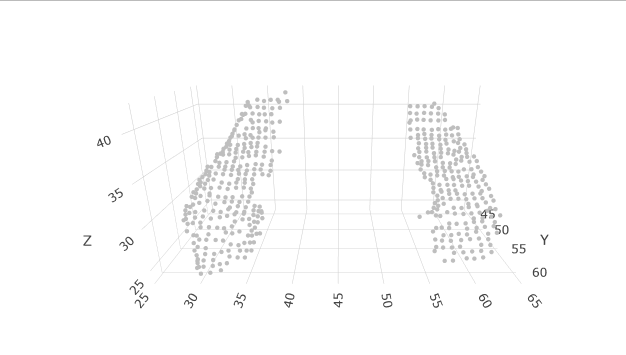} \\ 
        (a) Diagnosis × Subtype (SUVR)   & (b) Quadratic stage × Subtype (SUVR)\\
        \includegraphics[width=0.45\textwidth]{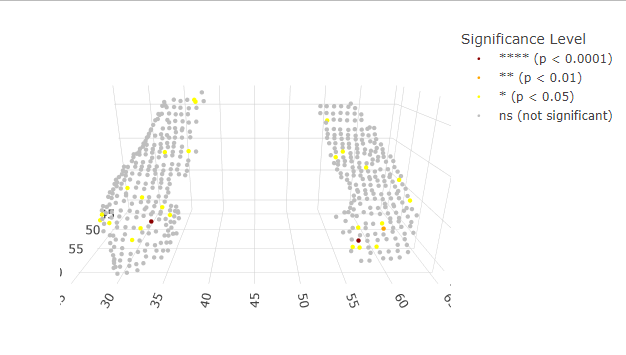}&
        \includegraphics[width=0.45\textwidth]{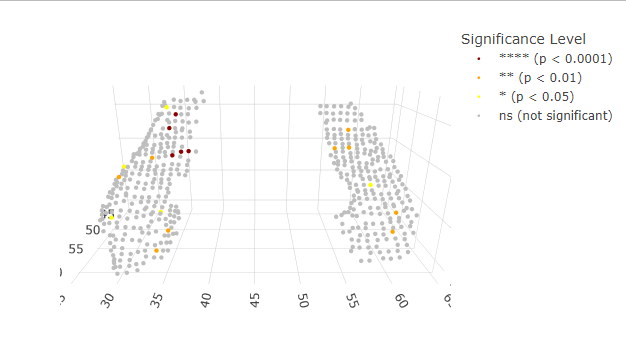} \\
        (c) Age × Subtype (Thickness)  & (d) Sex × Subtype (Thickness)\\
        \includegraphics[width=0.45\textwidth]{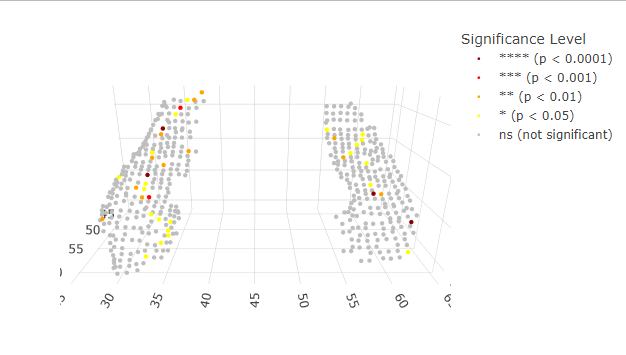}&
        \includegraphics[width=0.45\textwidth]{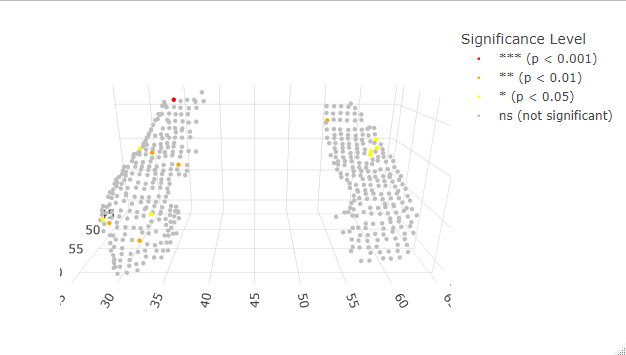} \\
        (e) Diagnosis × Subtype (Thickness)  & (f) Linear stage × Subtype (Thickness)\\
    \end{tabular}
\caption{
Significance maps for covariate-by-subtype interaction terms in the unified regression model. 
Each map displays surface regions where the effect of a covariate on tau deposition differs significantly between subtypes. 
(a)~Significance of the diagnosis effect interaction on SUVR intensity; 
(b)~Interaction significance for SuStaIn stage (quadratic term) on SUVR intensity; 
(c)~Interaction significance of age on positive projection thickness; 
(d)~Interaction significance of sex on positive projection thickness; 
(e)~Interaction significance of diagnosis on positive projection thickness; 
(f)~Interaction significance of SuStaIn stage (linear term) on positive projection thickness. All maps display $-{\log_{10}}(p)$ values from IPW-adjusted regression models, with multiple significance levels indicated by color intensity. 
Benjamini–Hochberg correction was applied across all vertices to control for multiple comparisons.}
\label{fig:sup_interaction}
\end{figure}

\begin{figure}[h]
    \centering
    \begin{tabular}{cc}
        \includegraphics[width=0.45\textwidth]{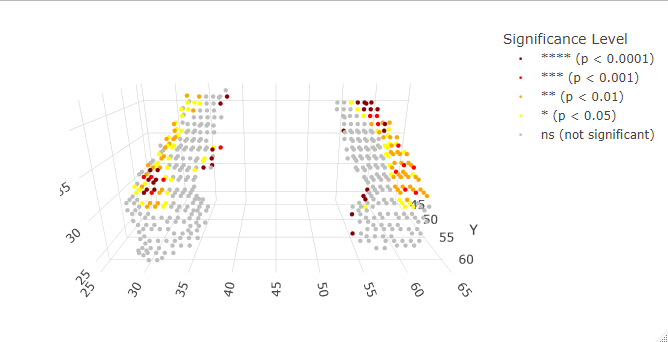}&
        \includegraphics[width=0.45\textwidth]{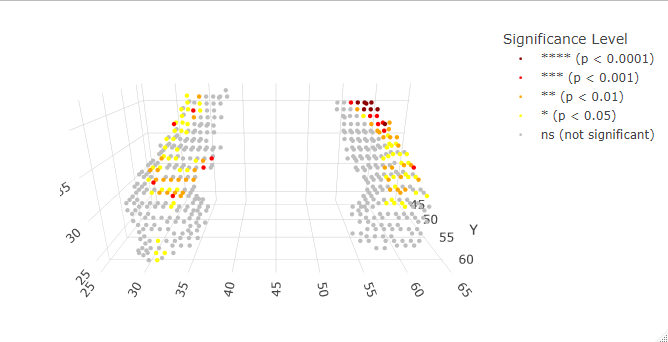} \\ 
        (a) Age effect (subtype 1)   & (b) Diagnosis effect (subtype 1)\\
        \includegraphics[width=0.45\textwidth]{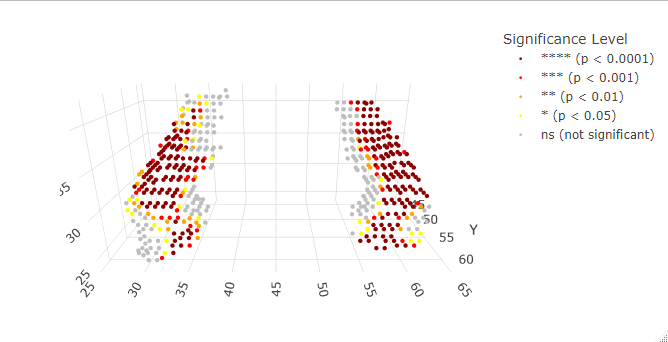}&
        \includegraphics[width=0.45\textwidth]{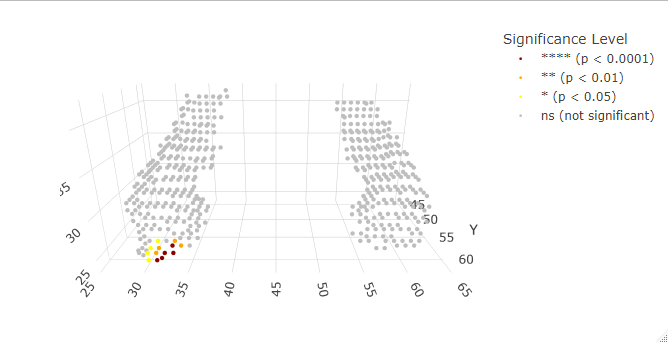} \\
        (c) Linear stage effect (subtype 1)  & (d) Quadratic stage effect (subtype 1)\\
    \end{tabular}
\caption{
Voxelwise regression significance maps for subtype 1, displayed in MNI coordinate space. Each map shows the spatial distribution of covariate effects on SUVR at individual voxel locations without thresholding or projection onto surface geometry. (a–d) depict the significance of regression coefficients for age, diagnosis, linear SuStaIn stage, and quadratic SuStaIn stage, respectively. Statistical testing was performed at each voxel using linear regression, and $p$-values were corrected for multiple comparisons using the Benjamini–Hochberg (BH) procedure. These maps provide a conventional voxelwise baseline for comparison with our surface-based modeling framework.
}
\label{fig:sup_voxel}
\end{figure}

\begin{figure}[h]
    \centering
    \begin{tabular}{cc}
        \includegraphics[width=0.45\textwidth]{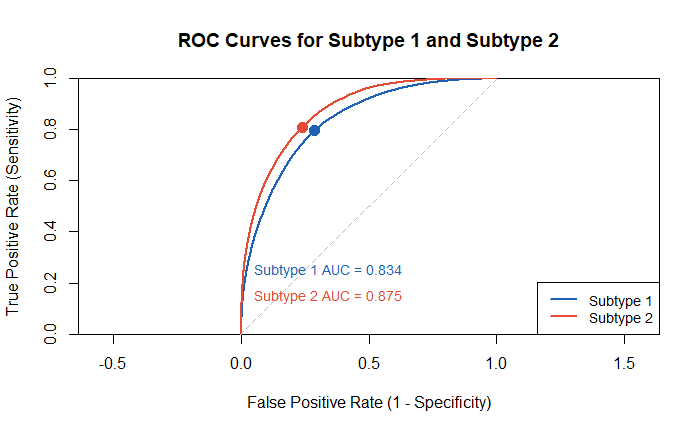} \\ 
        (a) ROC curves for tau coverage 
    \end{tabular}
    \caption{
Model-based prediction of tau deposition shapes across SuStaIn stages using two-stage regression. 
(a) ROC curves for pointwise logistic models of tau coverage in subtype 1 and subtype 2, evaluated across all selected surface points and subjects. 
The models achieved high discriminative performance (AUC = 0.834 for subtype 1, 0.875 for subtype 2).
}
\label{fig:prediction_ROC}
\end{figure}

\begin{figure}[h]
    \centering
    \begin{tabular}{cc}

        \includegraphics[width=0.45\textwidth]{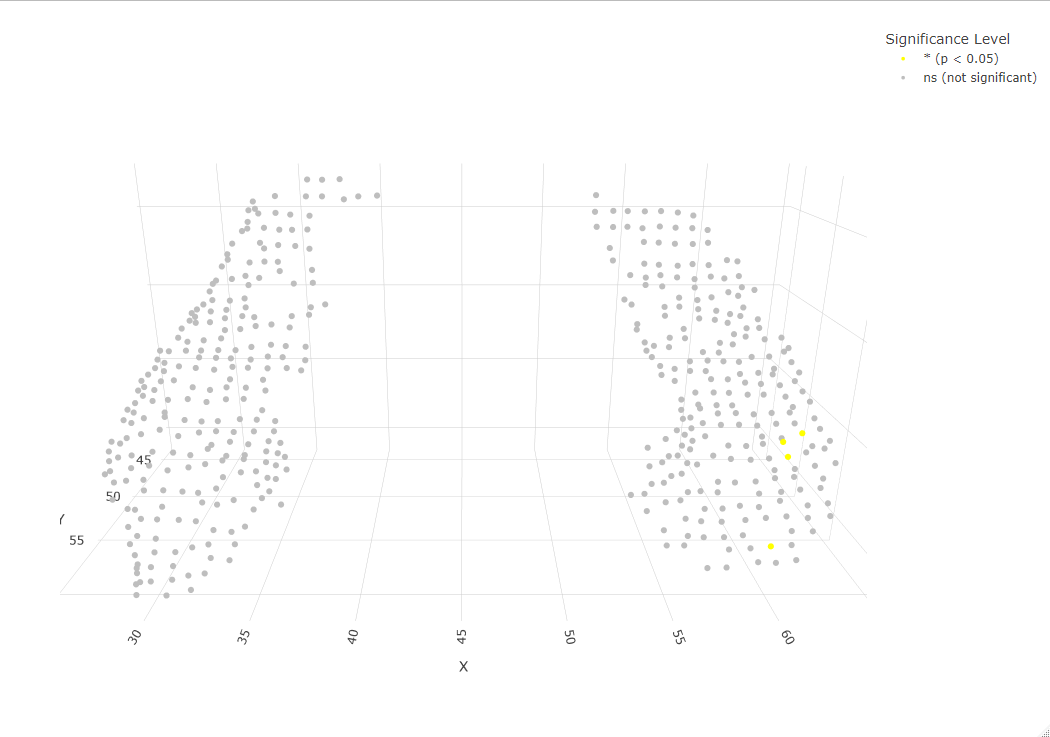} &
        \includegraphics[width=0.45\textwidth]{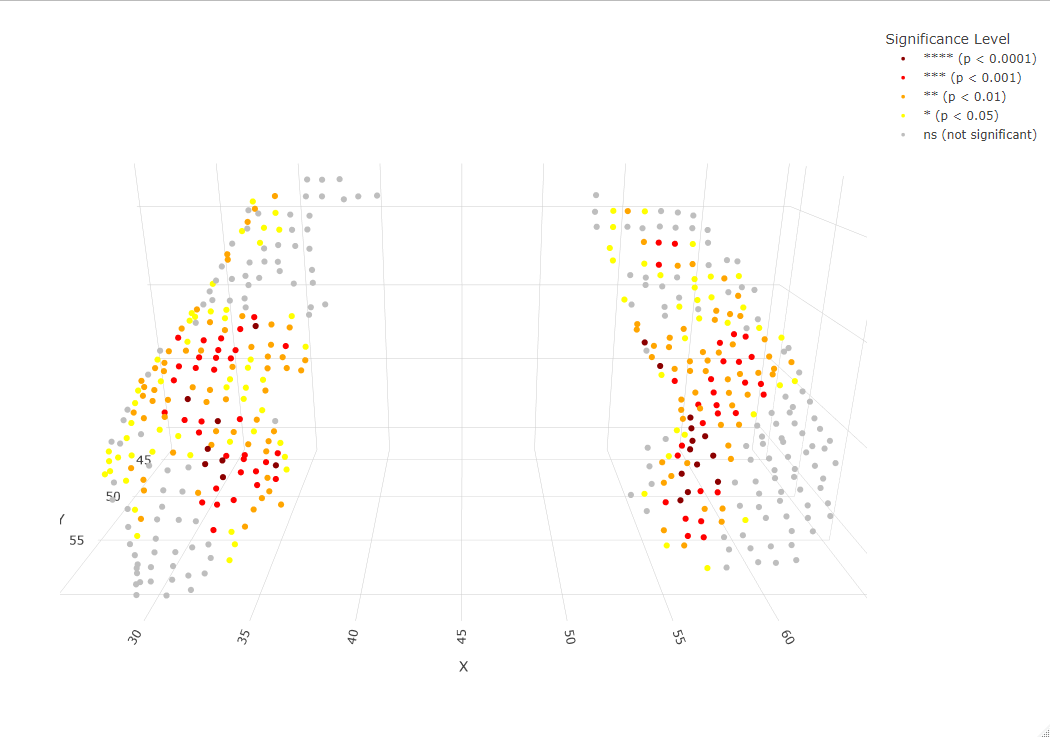} \\
        (a) Subject A (CN, negative) & (b) Subject A (CN, positive) \\
 
        \includegraphics[width=0.45\textwidth]{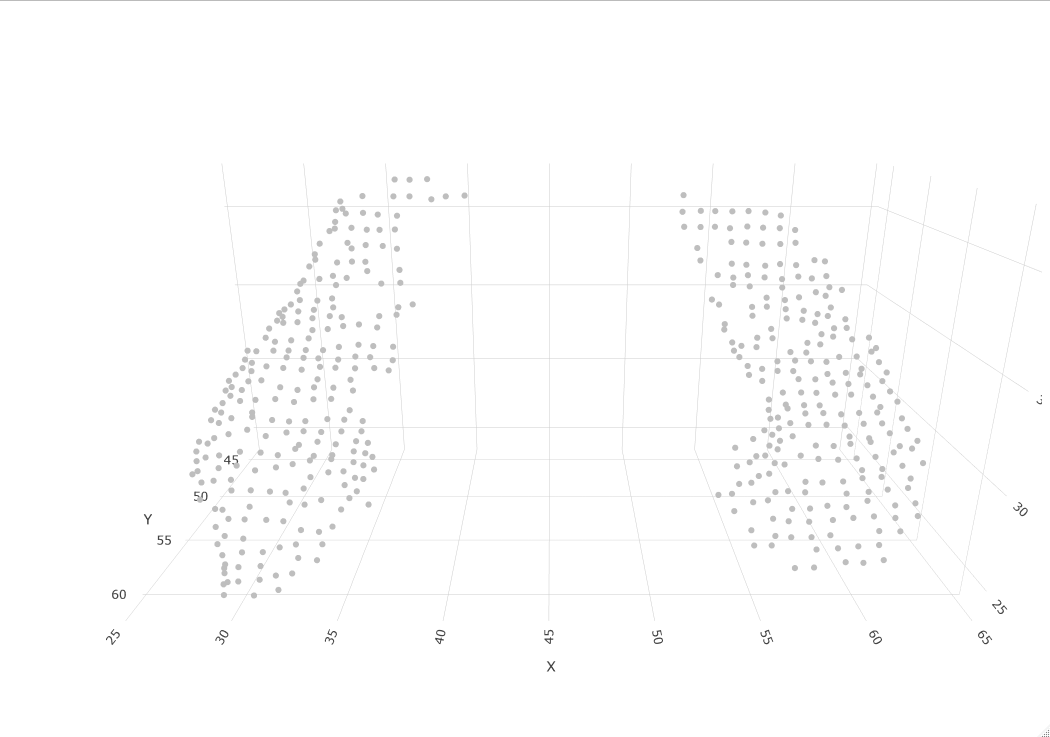} &
        \includegraphics[width=0.45\textwidth]{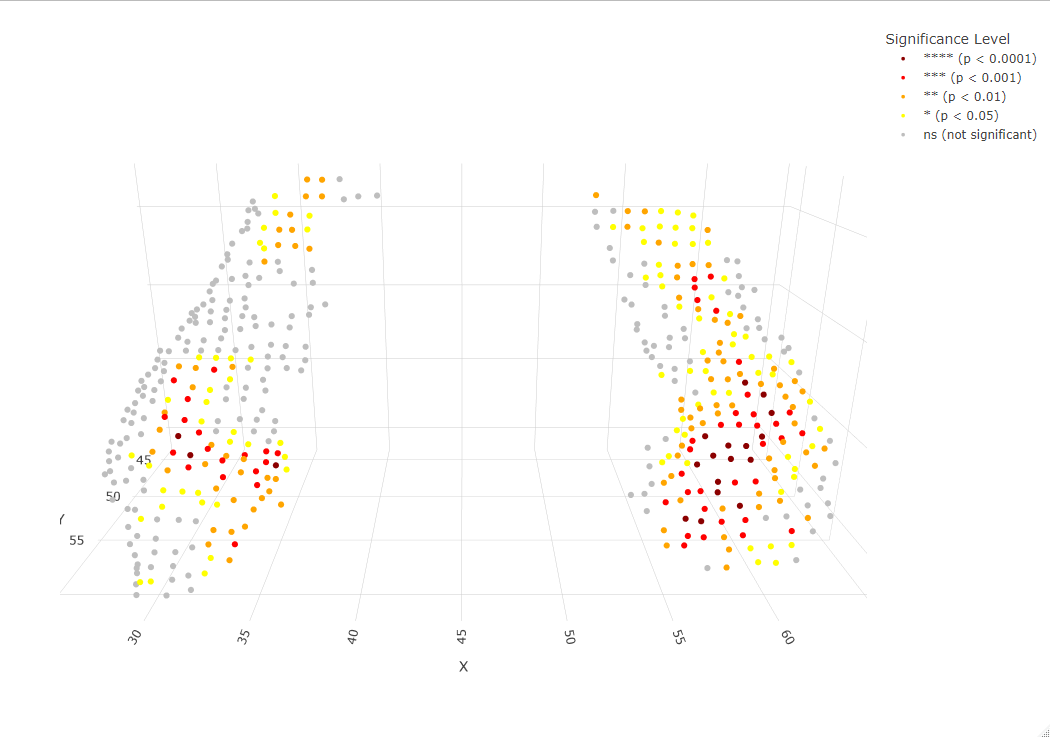} \\
        (c) Subject B (MCI, negative) & (d) Subject B (MCI, positive) \\

        \includegraphics[width=0.45\textwidth]{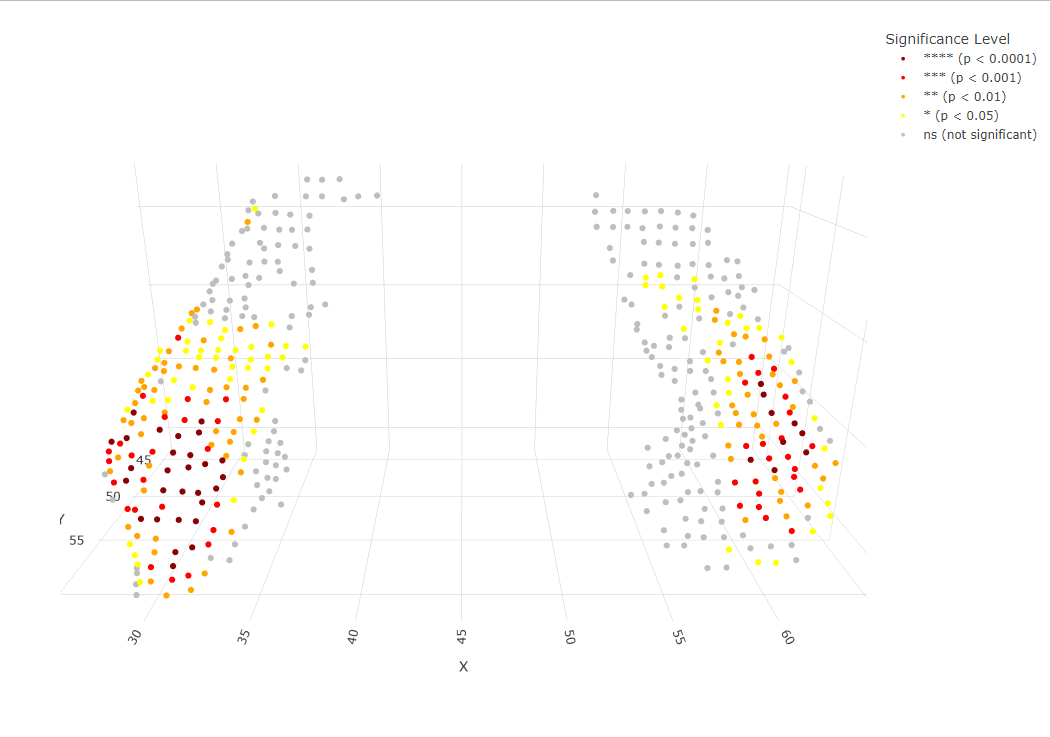} &
        \includegraphics[width=0.45\textwidth]{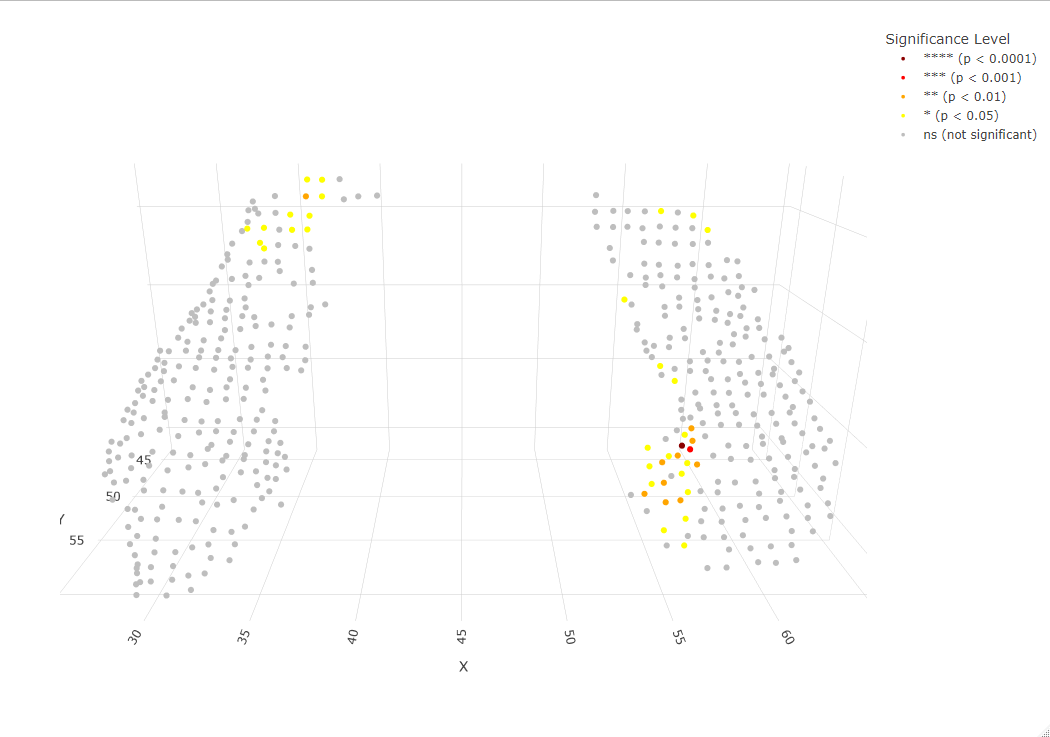} \\
        (e) Subject C (AD, negative) & (f) Subject C (AD, positive) \\
    
    \end{tabular}
     \caption{\textbf{Subject-Level Contamination Significance Maps.}
    Left: significance of negative contamination; Right: significance of positive contamination. 
    Participants are shown in order of increasing hippocampal tau burden. 
    Positive contamination is prominent in CN and MCI, whereas negative contamination emerges in AD.
    }
    \label{fig:supp_contam_examples}
\end{figure}

\section{External Validation using Amyloid Scans}

\subsection{Data Source and Preprocessing}

\paragraph{Sample characteristics}  
In the analysis, we included PET-MRI pairs from 611 participants from the ADNI study, each with T1-weighted MRI acquired within two years of the corresponding amyloid PET scan. Of these, 129 were cognitively normal (CN), 412 had mild cognitive impairment (MCI), and 70 were diagnosed with Alzheimer’s disease (AD). 
The sample included 276 males and 335 females, with a mean age of 74.6 years (SD = 7.8, range = 56.4–97.5 years). Table \ref{table:demographics} describes the general demographic characteristics by study group for the participants included in the final sample. 

\begin{table}[htbp]
\centering
\caption{Demographic characteristics of the participants included in the study, stratified by diagnostic group. Values are presented as mean (standard deviation) for continuous variables and count (percentage) for categorical variables. APOE4 carrier status was derived from APOE genotypes (Missing if either allele was NA/invalid; Carrier if A1=4 or A2=4; Non-carrier otherwise).}
\label{table:demographics}
\begin{tabular}{lcccc}
\toprule
 & \textbf{CN (N=129)} & \textbf{MCI (N=412)} & \textbf{AD (N=70)} & \textbf{Total (N=611)} \\
\midrule
\multicolumn{5}{l}{\textbf{Age (years)}} \\
\quad Mean (SD)         & 76.6 (7.1) & 73.7 (7.8) & 76.1 (8.0) & 74.6 (7.8) \\
\quad Median [Min, Max] & 76.7 [56.4, 92.0] & 73.4 [56.6, 97.5] & 77.4 [57.1, 91.4] & 74.9 [56.4, 97.5] \\
\addlinespace
\multicolumn{5}{l}{\textbf{Sex}} \\
\quad Female            & 66 (51.2\%) & 174 (42.2\%) & 36 (51.4\%) & 276 (45.2\%) \\
\quad Male              & 63 (48.8\%) & 238 (57.8\%) & 34 (48.6\%) & 335 (54.8\%) \\
\addlinespace
\multicolumn{5}{l}{\textbf{APOE $\epsilon$4 Carrier}} \\
\quad Non-carrier       & 99 (76.7\%) & 248 (60.2\%) & 24 (34.3\%) & 371 (60.7\%) \\
\quad Carrier           & 30 (23.3\%)  & 164 (39.8\%) & 46 (65.7\%) & 240 (39.3\%) \\
\quad Missing           & 0 (0\%)   & 0 (0\%) & 0 (0\%) & 0 (0\%) \\
\bottomrule
\end{tabular}
\end{table}

\paragraph{Image acquisition and preprocessing}  

All scans were pre-processed following the standard ADNI pipeline. Acquisition protocols for MRI and PET, as well as details on pre-processing procedures are described in detail at \texttt{https://adni.loni.usc.edu/}. Briefly, amyloid PET images were first co-registered to the corresponding native-space T1-weighted MRI, and then non-linearly warped to the MNI152 template space to ensure consistent anatomical alignment across subjects. For this analysis SUVR images were computed using the cerebellar gray matter as the reference region, applied uniformly across tracers (PiB/AV45/FBB), and partial volume correction was applied to reduce spill-over effects. A random subset of images from each scanner model was visually inspected to verify registration quality and confirm the absence of major motion artifacts. To account for potential site-related variability, we applied the neuroCombat algorithm to correct for scanner- and protocol-induced batch effects. Scans were grouped by scanner model, with rare models (fewer than five scans) merged by manufacturer. Age, sex, and diagnosis were included as biological covariates in the harmonization model to preserve meaningful variance while removing non-biological noise.

\paragraph{Hippocampal Structure and Amyloid Signal Definition}  \label{sec: atlas}

For spatial localization, hippocampal geometry was defined using the MNI152-space T1-weighted MRI Automated Anatomical Labeling (AAL) atlas. The hippocampal region in this atlas was used to construct a medial surface representation, which served as a shared spatial surface for projecting amyloid PET signals. Because hippocampal A$\beta$ signal is typically low and PET measurements are confounded by adjacent choroid-plexus uptake, we treat this as an external validation of the projection pipeline rather than a canonical amyloid topography analysis. To identify regions with elevated amyloid deposition, we applied a fixed thresholding procedure to each participant’s PET SUVR image. Voxels with SUVR values exceeding 1.1 were considered amyloid-positive, this cutoff was chosen from our cohort-level SUVR distributional analysis. This subject specific binary mask was then projected onto the medial hippocampal surface for downstream shape based analysis. The SuStaIn modeling followed the same implementation as in the tau analysis, with the amyloid mask defined by the 1.1 SUVR cutoff.

\subsection{Results}

\paragraph{SuStaIn-Derived Subtypes and Disease Staging} As an external pipeline validation on hippocampal projections, we applied the same SuStaIn implementation used for tau to the amyloid data. To avoid overinterpretation, we did not enforce correspondence between the amyloid derived subtype labels and the canonical tau phenotypes (i.e., limbic-dominant, posterior occipitotemporal, parietal-dominant/MTL-sparing, left-temporal); labels here are analysis specific. Subject specific masks used a fixed cutoff of $SUVR=1.1$; participants with no hippocampal voxels with $SUVR \geq 1.1$ were labeled stage 0 (subtype 0). The cohort split into subtype 0 ($n=312$) and four nonzero subtypes ($n=101, 98, 88, 12$ for subtypes 1--4). Subtypes 1, 2 and 3 span a wide range of stages and include mostly CN and MCI individuals, while subtype 4 is smaller and more skewed toward later stages and AD diagnosis (Fig.~\ref{fig:spatial_coverage_num}). Given the limited sample size and reduced clinical variability of subtype 4, all subsequent analyses focus on subtypes 1, 2, and 3, which represent the dominant patterns of hippocampal amyloid accumulation in this cohort.

\begin{figure}[htbp]
    \centering
    \begin{tabular}{cc}
        \includegraphics[width=0.45\textwidth]{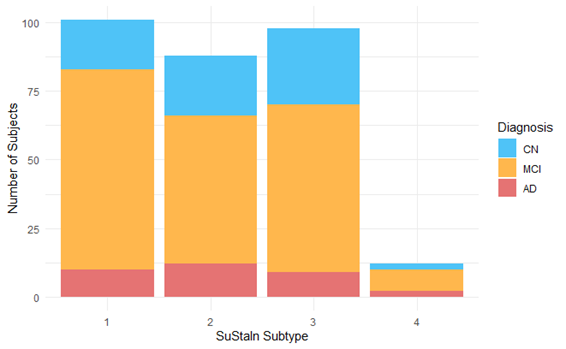}&
        \includegraphics[width=0.45\textwidth]{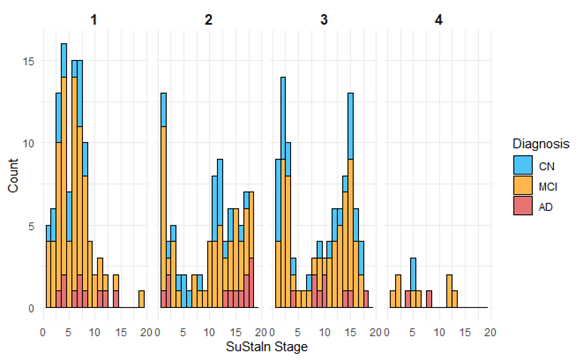} \\
        (a) Diagnosis within SuStaIn subtypes  & (b) Stage across SuStaIn subtypes  \\
        
    \end{tabular}
   \caption{Overview of SuStaIn-derived subtypes  (a) Diagnosis composition (CN, MCI, AD) within each subtype, shown as a stacked bar plot.  (b) Distribution of SuStaIn stages within each subtype, stratified by diagnosis.  Subtypes 1, 2 and 3 are predominantly early to mid-stage with a higher proportion of CN and MCI cases, while subtypes 4 are mid to later stage with more MCI and AD cases. 
    }
    \label{fig:spatial_coverage_num}
\end{figure}

\paragraph{Pointwise Coverage of Amyloid Deposition on the Hippocampal Surface}

Similar to the tau analysis, we examined spatial coverage patterns using the logistic regression model. The number of scans in which each surface point was covered is visualized in (Fig.~\ref{fig:coverage_diagnosis_linear_quadratic} a-c) for subtype 1-3 respectively. In all plots, the surface is displayed with anterior at the bottom and posterior at the top, with the right hippocampus on the left and the left hippocampus on the right, matching a brain orientation facing the viewer.
Coverage is spatially non-uniform with focal clusters on the hippocampal surface. The right hippocampus generally shows higher coverage than the left, with peaks centered in the lateral/central body. Subtypes 1 and 3 produce the right-dominant pattern and subtype 2 shows a similar but more spatially restricted hotspot.

We next evaluated how coverage patterns were modulated by covariates. (Fig.~\ref{fig:coverage_diagnosis_linear_quadratic} d-f) display significance maps for the logistic regression coefficients associated with diagnosis and SuStaIn stage in all three subtypes. Diagnosis shows no significance or spatially distinct effect. Thus, within subtypes, clinical diagnosis is not a reliable predictor of suprathreshold hippocampal amyloid coverage. 
SuStaIn stage was also included in the model to account for variation along the disease progression axis. To reflect its ordinal nature (20 levels), stage was encoded as a second-order polynomial. Both the linear and quadratic components are shown in (Fig.~\ref{fig:coverage_diagnosis_linear_quadratic} g-l). The linear component (Fig.~\ref{fig:coverage_diagnosis_linear_quadratic} g–i) indicates that advancing stage increases the probability of suprathreshold amyloid coverage as effects in subtypes 2 and 3 show strong signals over the right lateral/mid-anterior hippocampal surface with smaller patches on the left (medial/posterior); whereas subtype 1 shows weaker signals in the right lateral/posterior and left anterior regions. By contrast, the quadratic term (Fig.~\ref{fig:coverage_diagnosis_linear_quadratic} j–l) shows no significant effect.

\begin{figure}[htbp]
    \centering
    \setlength{\tabcolsep}{2pt} % tighten column gaps; adjust if needed
    \begin{tabular}{@{}ccc@{}}
        % Row 1: Coverage
        \includegraphics[width=0.31\textwidth]{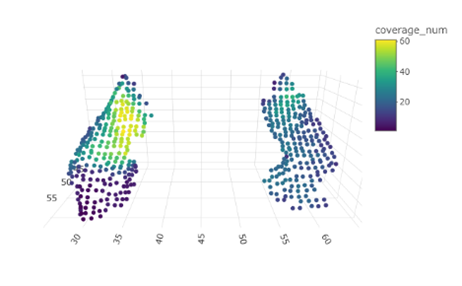} &
        \includegraphics[width=0.31\textwidth]{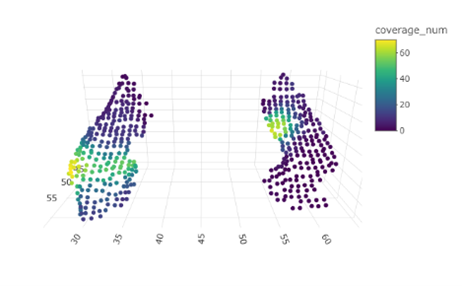} &
        \includegraphics[width=0.31\textwidth]{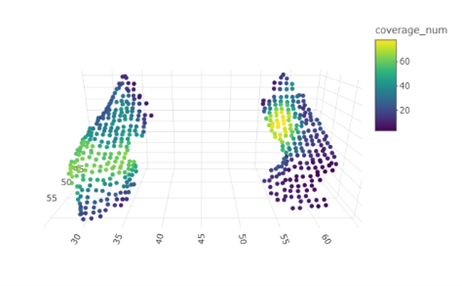} \\
        \small (a) Coverage map (subtype 1) & \small (b) Coverage map (subtype 2) & \small (c) Coverage map (subtype 3) \\
        % Row 2: Diagnosis 
        \includegraphics[width=0.31\textwidth]{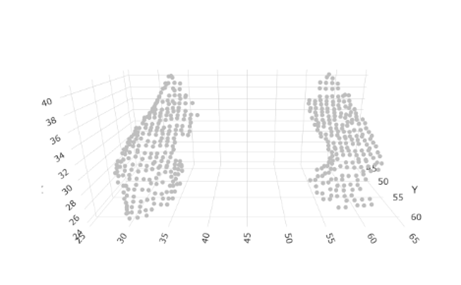} &
        \includegraphics[width=0.31\textwidth]{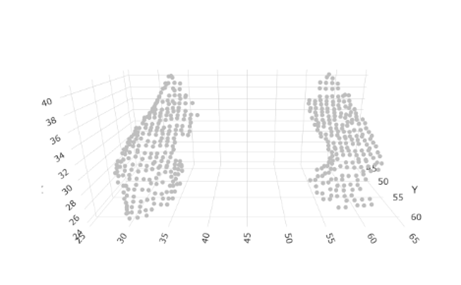} &
        \includegraphics[width=0.31\textwidth]{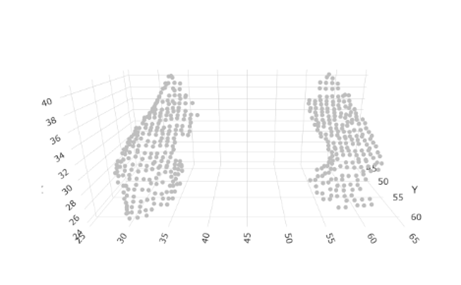} \\
        \small (d) Diagnosis effect (subtype 1) & \small (e) Diagnosis effect (subtype 2) & \small (f) Diagnosis effect (subtype 3) \\
        % Row 3: Linear #2
        \includegraphics[width=0.31\textwidth]{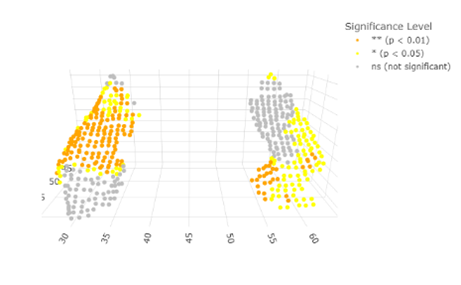} &
        \includegraphics[width=0.31\textwidth]{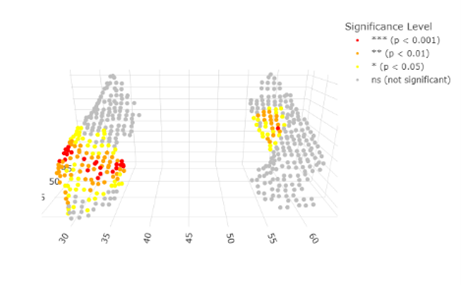} &
        \includegraphics[width=0.31\textwidth]{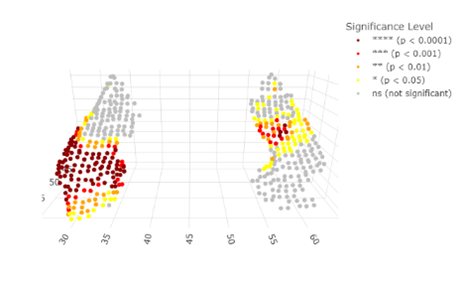} \\
        \small (g) Linear stage effect (subtype 1) & \small (h) Linear stage effect (subtype 2) & \small (i) Linear stage effect (subtype 3) \\
        % Row 4: Quadratic
        \includegraphics[width=0.31\textwidth]{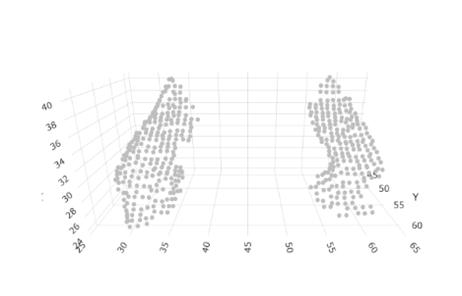} &
        \includegraphics[width=0.31\textwidth]{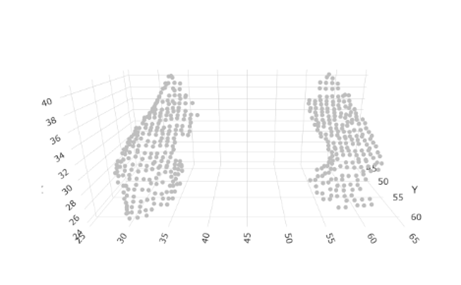} &
        \includegraphics[width=0.31\textwidth]{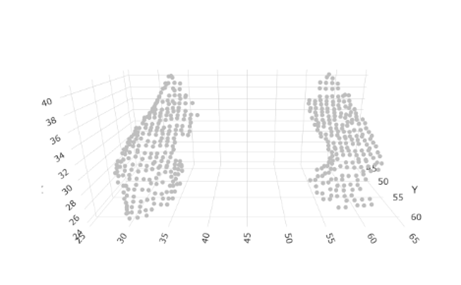} \\
        \small (j) Quadratic stage effect (subtype 1) & \small (k) Quadratic stage effect (subtype 2) & \small (l) Quadratic stage effect (subtype 3)
    \end{tabular}
    \caption{Coverage and significance maps for covariate effects on suprathreshold amyloid signal across the hippocampal surface. Panels (a-c) display the number of scans showing suprathreshold signal $SUVR \geq 1.1$ at each surface location for subtype 1, subtype 2, and subtype 3 respectively. Panels (d–f) show no significant diagnosis effect on amyloid coverage, estimated using IPW-adjusted logistic regression. Panels (g–i) depict the significance of the linear SuStaIn stage effect, and panels (j–l) depict the quadratic SuStaIn stage effect, which are not significant. Here, the “linear” and “quadratic”
components correspond to the first two orthogonal polynomial terms.}
    \label{fig:coverage_diagnosis_linear_quadratic}
\end{figure}

\paragraph{Covariate Effects on Amyloid Deposition Intensity (SUVR)}

We evaluated the effects of age, diagnosis, and SuStaIn stage on hippocampal amyloid SUVR, separately within each subtype. The significance maps are shown in (Fig.~\ref{fig:age_diagnosis_linear_quadratic_effect}). For age related effects (Fig.~\ref{fig:age_diagnosis_linear_quadratic_effect} a-c) no surface locations are significant in subtype 1, and only a few isolated vertices appear in subtypes 2 and 3 with small, inconsistent signs and no coherent spatial pattern. Diagnosis effects were predominantly observed in subtype 3 (Fig.~\ref{fig:age_diagnosis_linear_quadratic_effect} d-f). Significant regions are localized to the right anterior-to-posterior medial surface and no effects are evident on the left hippocampus. In subtype 1 and 2 there were no significant regions indicating no spatially coherent diagnosis effect on hippocampal amyloid SUVR in these subtypes. Linear SuStaIn stage effects showed strong and widespread significance in subtypes 1 and 3 (Fig.~\ref{fig:age_diagnosis_linear_quadratic_effect} g–i), with clusters concentrated along the right hippocampal medial surface and extending anterior–to–posterior. Subtype 2 exhibits scattered, small clusters. In Quadratic stage terms (Fig.~\ref{fig:age_diagnosis_linear_quadratic_effect} j–l) a few localized patches appear in subtype 1 and 2 while subtype 3 show no statistically significant vertices.

\begin{figure}[htbp]
    \centering
    \setlength{\tabcolsep}{2pt} % tighten column gaps; adjust if needed
    \begin{tabular}{@{}ccc@{}}
        % Row 1: Age
        \includegraphics[width=0.31\textwidth]{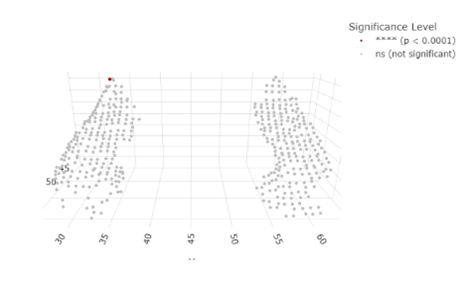} &
        \includegraphics[width=0.31\textwidth]{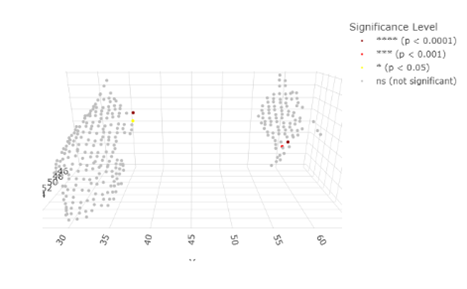} &
        \includegraphics[width=0.31\textwidth]{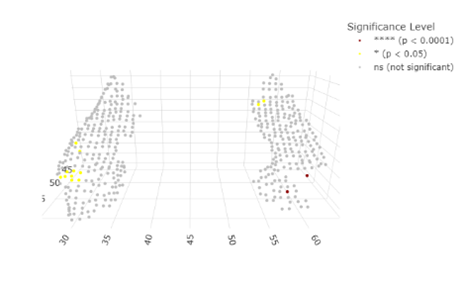} \\
        \small (a) Age effect (subtype 1) & \small (b) Age effect (subtype 2) & \small (c) Age effect (subtype 3) \\
        % Row 2: Diagnosis #1
        \includegraphics[width=0.31\textwidth]{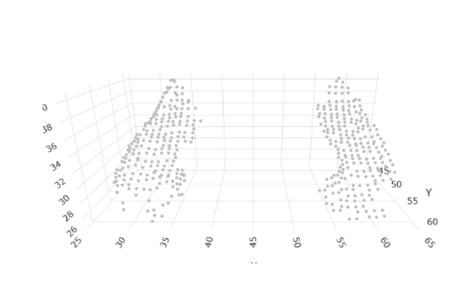} &
        \includegraphics[width=0.31\textwidth]{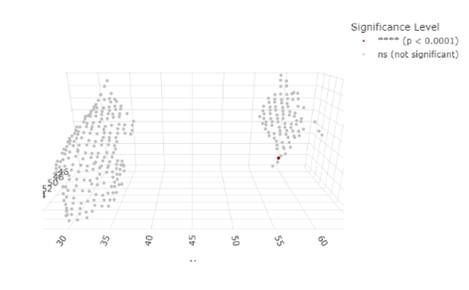} &
        \includegraphics[width=0.31\textwidth]{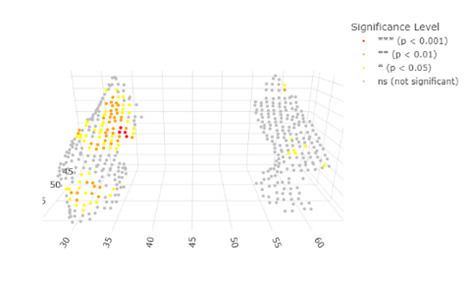} \\
        \small (d) Diagnosis effect (subtype 1) & \small (e) Diagnosis effect (subtype 2) & \small (f) Diagnosis effect (subtype 3) \\
        % Row 3: Linear
        \includegraphics[width=0.31\textwidth]{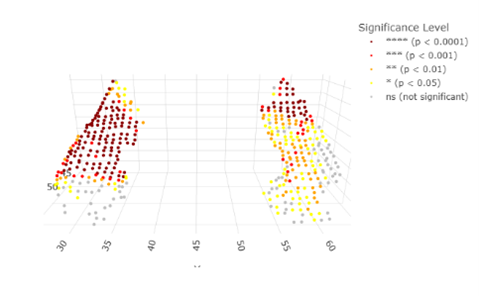} &
        \includegraphics[width=0.31\textwidth]{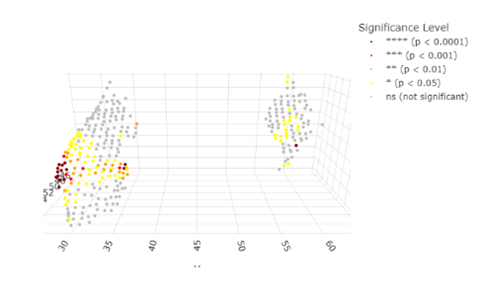} &
        \includegraphics[width=0.31\textwidth]{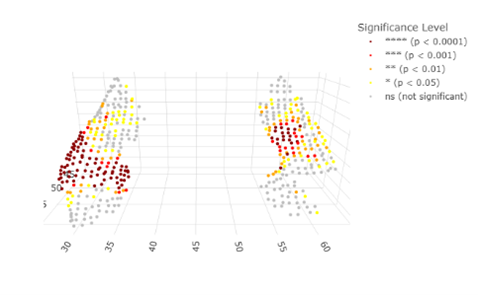} \\
        \small (g) Linear stage effect (subtype 1) & \small (h) Linear stage effect (subtype 2) & \small (i) Linear stage effect (subtype 3) \\
        % Row 4: Quadratic
        \includegraphics[width=0.31\textwidth]{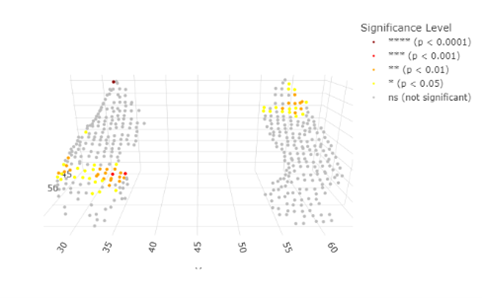} &
        \includegraphics[width=0.31\textwidth]{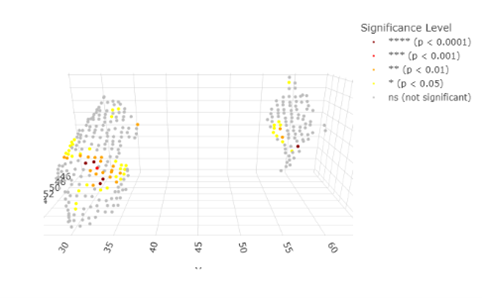} &
        \includegraphics[width=0.31\textwidth]{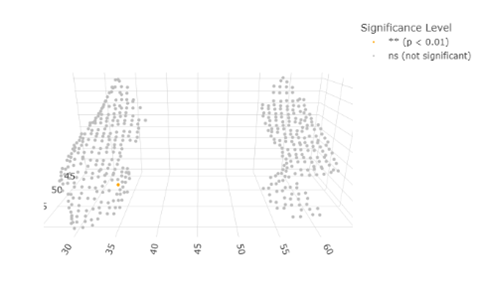} \\
        \small (j) Quadratic stage effect (subtype 1) & \small (k) Quadratic stage effect (subtype 2) & \small (l) Quadratic stage effect (subtype 3)
    \end{tabular}
    \caption{Significance maps of covariate effects on hippocampal amyloid SUVR. (a–c) Age-related effects show a very tiny significant cluster in the right lateral part of hippocampus of subtype 3 with few scattered vertices in subtype 2. (d–f) Diagnosis related effects are stronger in subtype 3 and non-significant in subtypes 1 and 2. (g–l) SuStaIn stage, linear effect is widespread in subtype 1, 3 and Subtype 2 exhibits scattered, small clusters. Quadratic stage terms show a few localized patches in subtype 1 and 2 while subtype 3 is statistically non-significant. Here, we excluded vertices whose per vertex IPW SUVR model could not be estimated.}
    \label{fig:age_diagnosis_linear_quadratic_effect}
\end{figure}

\paragraph{Stage-Dependent Effects on Tau Deposition Thickness}

To capture shape-level changes in amyloid pathology beyond intensity or coverage, we analyzed a geometric measure of deposition thickness based on projection distance. Linear stage effects were observed in subtypes 2 and 3 and across both projection directions whereas subtype 1 shows insignificant effect (Fig.~\ref{fig:negative_positive_linear_quadratic_effect} a-f). In subtype 2 and 3, the spatial pattern of significance was nearly identical between the positive and negative features, indicating that amyloid thickness increases occur symmetrically around the principal surface. Quadratic effects were weak (Fig.~\ref{fig:negative_positive_linear_quadratic_effect} g–l), a few localized data points were observed with no spatial pattern. 

\begin{figure}[htbp]
    \centering
    \setlength{\tabcolsep}{1pt} % tighten column gaps; adjust if needed
    \begin{tabular}{@{}ccc@{}}
        % Row 1:
        \includegraphics[width=0.28\textwidth]{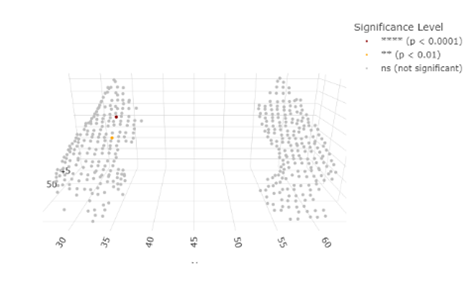} &
        \includegraphics[width=0.31\textwidth]{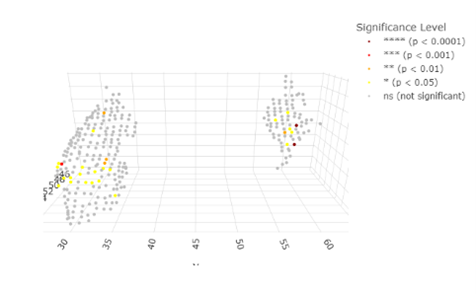} &
        \includegraphics[width=0.31\textwidth]{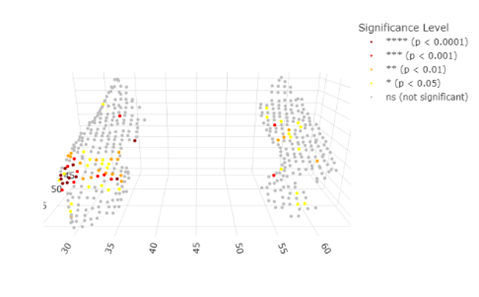} \\
        \small (a) Negative linear effect (subtype 1) & \small (b) Negative linear effect (subtype 2) & \small (c) Negative linear effect (subtype 3) \\
        % Row 2: 
        \includegraphics[width=0.31\textwidth]{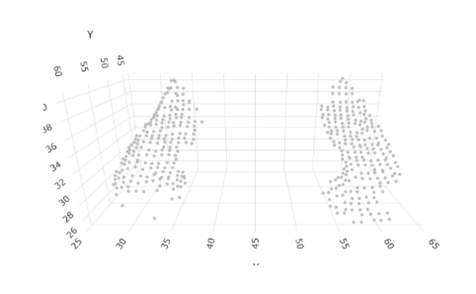} &
        \includegraphics[width=0.31\textwidth]{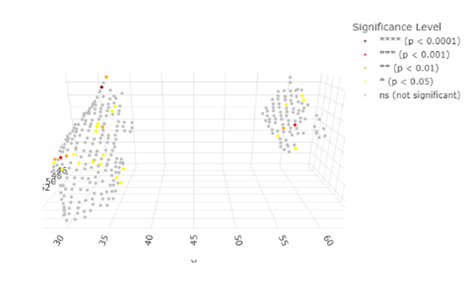} &
        \includegraphics[width=0.31\textwidth]{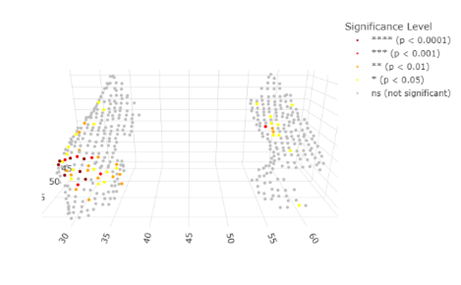} \\
        \small (d) Positive linear effect (subtype 1) & \small (e) Positive linear effect (subtype 2) & \small (f) Positive linear effect (subtype 3) \\
        % Row 3:
        \includegraphics[width=0.31\textwidth]{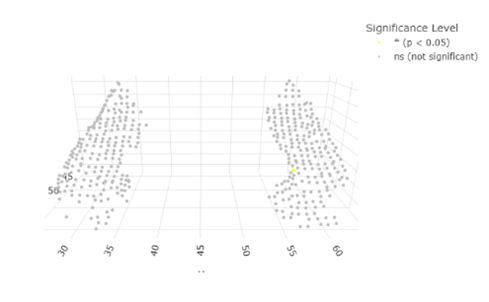} &
        \includegraphics[width=0.31\textwidth]{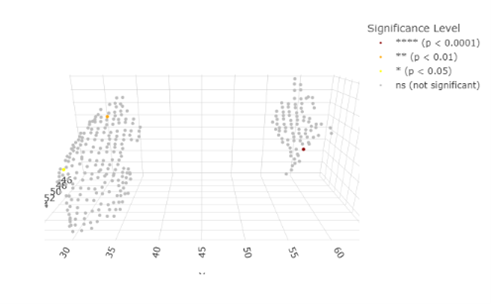} &
        \includegraphics[width=0.31\textwidth]{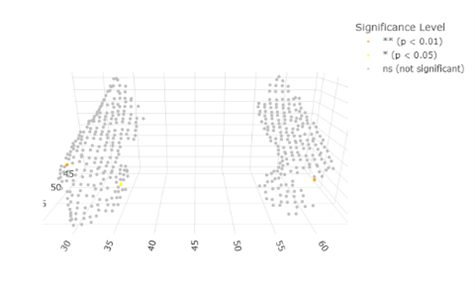} \\
        \small (g) Negative Quadratic effect (subtype 1) & \small (h) Negative Quadratic effect (subtype 2) & \small (i) Negative Quadratic effect (subtype 3) \\
        % Row 4:
        \includegraphics[width=0.31\textwidth]{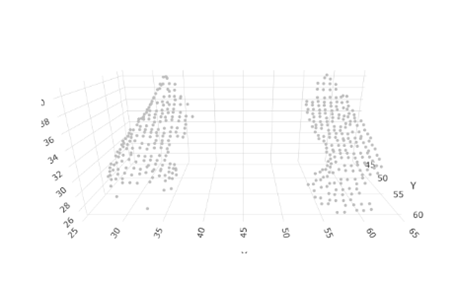} &
        \includegraphics[width=0.31\textwidth]{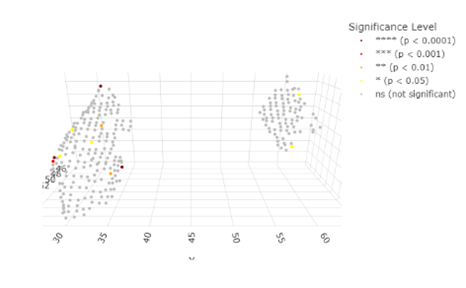} &
        \includegraphics[width=0.31\textwidth]{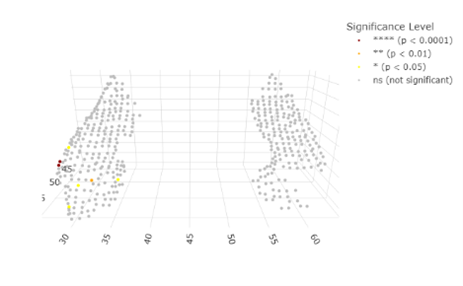} \\
        \small (j) Positive Quadratic effect (subtype 1) & \small (k) Positive Quadratic effect (subtype 2) & \small (l) Positive Quadratic effect (subtype 3)
    \end{tabular}
    \caption{Significance maps of SuStaIn stage effects on hippocampal amyloid deposition thickness, separated by subtype, projection direction, and polynomial term. Each panel shows results from an IPW-adjusted regression model fit within a specific subtype. Panels (a–f) correspond to negative-direction projection distances; (g–l) show positive-direction thickness. All maps display -log10(p) values thresholded at multiple significance levels after BH correction for multiple comparisons. Subtype labels are indicated in parentheses for consistency with other figures. Here, we excluded vertices whose per vertex IPW SUVR model could not be estimated.}
    \label{fig:negative_positive_linear_quadratic_effect}
\end{figure}

\end{document}
